# Supplementary material for: On globally invariant Euler--Lagrange equations for curves
Source: arXiv:2601.06985 ancillary file (2026-01-11)
Supplement: Supplementary file 1 [file Supplement_0_EL_equations_MV.pdf]

**Supplement to the article: 'On globally invariant Euler--Lagrange equations for curves' by Boris Kruglikov, Eivind Schneider, Wijnand Steneker.**
**Date: 07.01.2026**

**Description of Maple file:** We compute the invariant Euler--Lagrange equations for G-invariant variational problems for the following Lie group actions: Moebius2D, Projective2D, Euclidean3D, Conformal3D and Euclidean4D. In this supplementary Maple worksheet, we make extensive use of moving frame methods as developed by Kogan--Olver. This entails using an invariantization map together with a local cross-section & prolonged Lie algebra action. We use the DifferentialGeometry package by I. Anderson.

The ordinary Euler--Lagrange equations can be computed as EL = W*[Astar(Eulerian) - Bstar (Hamiltonian)] = 0, where W is a matrix relative invariant. We compute the matrix relative invariant W using explicit expressions for invariant contact forms of order 0 constructed from the symbols of the scalar differential invariants cf. section 2.2. These can be related to invariantizations of the standard contact forms by evaluating on the cross-section. (In order to check our results, we apply the operators Astar and Bstar to explicit invariant Lagrangians and compare the results with coordinate computations of the invariant EL eqs as well as compare with known examples in the literature.)

In [Kogan--Olver2001] the following question was raised: "*Are there examples of invariant variational problems all of whose extremals are singular, and hence cannot be expressed in terms of the (absolute) differential invariants?*". We show that the answer to this question is positive by example of conformal geodesics for the group G = Conf(3D) and the conformal torsion functional: the invariant EL equations are given by {0 = 0, -1 = 0}, which imply that there are no regular extremals. Computing W for Conf (3D) and multiplying it with the invariant EL vector [0,1]^T then give the (unparametrized) conformal geodesic equations.

The code follows closely the steps indicated in the algorithm in section 2.6.
In this code we do not implement the invariant horizontal forms ϖ and invariant contact forms ι(θ) as DG objects, and instead use abstract symbols in many places. This means we do not have access to tensor operations such as wedge product, and so we have to compute components of tensors instead. (E.g. The minus sign in expression for B is a consequence of wedge product.)

**Notation:**
Invariants: (e.g.) kappa (explicit coordinate expression), K (symbol) and K[0] (dependent variable in Maple notation, index in square bracket denotes number of differentiations wrt the invariant derivation)
Invariant horizontal form: varpi (only used as a symbol)
Invariantization of theta^y_j: iota_theta_y||j (symbol) *and* ICy||j[0] (dependent variable in Maple notation, index in square bracket denotes number of differentiations wrt the invariant derivation)
Invariant vertical derivative of ϖ is encoded by computing the invariant contact form B in the expression dv(ϖ) = B ∧ ϖ.

>

# Moebius 2D

```
> restart : with(DifferentialGeometry) : with(LieAlgebras) : with(Tensor) : with(GroupActions) :
    with(Tools) : Preferences("ShowFramePrompt",'false') : interface(warnlevel = 0) :
```

```
with(LinearAlgebra) : with(PDETools) : with(JetCalculus) : with(ArrayTools) :
Preferences("JetNotation", "JetNotation2") :
> DGsetup([x], [y], E, 12) : totalD := evalDG(D_x + add(y[i + 1] D_y[i], i = 0 ..10 )) :
  contact_forms := [seq(dy[i] − y[i + 1] dx, i = 0 ..8)] :
  # jet bundle, total derivative, contact forms
```

**Lie algebra of Moebius group:**

> $moeb := evalDG\left(\left[D\_x, D\_y[0], x\,D\_y[0] - y[0]\,D\_x,\ x\,D\_x + y[0]\,D\_y[0]\ ,\ \frac{1}{2}\cdot(x^2 + y[0]^2)\,D\_x - x\cdot(x\,D\_x + y[0]\,D\_y[0]),\ \frac{1}{2}\cdot(x^2 + y[0]^2)\,D\_y[0] - y[0]\cdot(x\,D\_x + y[0]\,D\_y[0]),\ \right]\right) : g := map(Prolong, moeb, 10) : r := nops(moeb) :$

**Local invariants:**

> $\ell := \left(1 + y_1^2\right)^{\frac{1}{2}} : \kappa := \frac{y_2}{\ell^3} : Ts := f \to simplify\left(\frac{1}{\ell}\ TotalDiff(f, 1)\right) : \kappa 0 := \kappa$ :**for** $i$ **to** 6 **do** $\kappa \| i := Ts\left(\kappa \| (i-1)\right)$:**od**:

> $q := \frac{4\,\kappa 1\,\kappa 3 - 4\,\kappa 0^2\,\kappa 1^2 - 5\,\kappa 2^2}{\kappa 1^3}$ : *# Moebius curvature*

> sigma := $f \to$ sqrt($kappa1$)$^{-1} \cdot \ell^{-1}$ $TotalDiff(f, x)$ : *# invariant derivation*
> $nabla := f \to q1$ sigma($f$) : *# global invariant derivation*

> $q0 := q$ : **for** $k$ **from** 1 **to** 7 **do** $q \| k :=$ sigma($simplify(q \| (k-1), symbolic)$):**od**:

> $seq(simplify(LieDerivative(Prolong(moeb[i], 10), [q, q1, q2, q3])), i = 1 ..6)$
*# checking that q, q_sigma, q_2sigma, q_3sigma are Moebius-invariant*

$$[0, 0, 0, 0], [0, 0, 0, 0], [0, 0, 0, 0], [0, 0, 0, 0], [0, 0, 0, 0], [0, 0, 0, 0] \quad (1.1)$$

# Computing cross-section:

> $V := evalDG(add(\ a \| i \cdot g[i]\ \ \ , i = 1 ..r)\ ) :$

> $LieDerivative(V, x)$

$$-a6\,x\,y_0 - \frac{1}{2}\ a5\,x^2 + \frac{1}{2}\ a5\,y_0^2 - a3\,y_0 + a4\,x + a1 \quad (1.1.1)$$

> $eval(LieDerivative(V, [x, y[0], ]), [\ ])$
*# We can set first three coordinates equal to zero by using translations, i.e., a1 = a2 = 0*

$$\left[-a6\,x\,y_0 - \frac{1}{2}\ a5\,x^2 + \frac{1}{2}\ a5\,y_0^2 - a3\,y_0 + a4\,x + a1,\ \frac{1}{2}\ a6\,x^2 - \frac{1}{2}\ a6\,y_0^2 - a5\,x\,y_0 + a3\,x + a4\,y_0 + a2\right] \quad (1.1.2)$$

> $eval(LieDerivative(V, [x, y[0]]), [\ x = 0, y[0] = 0,\ a1 = 0, a2 = 0,\ ])$

$$[0, 0] \quad (1.1.3)$$

> $eval(LieDerivative(V, [y[1], ]),\ [x = 0, y[0] = 0, y[1] = 0, a1 = 0, a2 = 0, a3 = 0])$

$$[0] \quad (1.1.4)$$

```
> eval(LieDerivative(V, [y[2], ]), [x = 0, y[0] = 0, y[1] = 0, y[2] = 0, a1 = 0, a2 = 0, a3 = 0,
     a6 = 0])
```

$$[0] \quad (1.1.5)$$

```
> eval(LieDerivative(V, [y[3], ]), [x = 0, y[0] = 0, y[1] = 0, y[2] = 0, y[3] = 1, a1 = 0, a2 = 0,
     a3 = 0, a6 = 0, a4 = 0])
```

$$[0] \quad (1.1.6)$$

```
> eval(LieDerivative(V, [y[4], ]), [x = 0, y[0] = 0, y[1] = 0, y[2] = 0, y[3] = 1, y[4] = 0, a1
     = 0, a2 = 0, a3 = 0, a6 = 0, a4 = 0, a5 = 0])
```

$$[0] \quad (1.1.7)$$

**Cross-section:**

```
> cs0 := [x = 0, y[0] = 0, y[1] = 0, y[2] = 0, y[3] = 1, y[4] = 0]; eval([q, q1], cs0)
     # q is invariantization of 4y_5, q1 is invariantization of 4y_6.
```

$$cs0 := [x = 0, y_0 = 0, y_1 = 0, y_2 = 0, y_3 = 1, y_4 = 0]$$

$$[4\,y_5, 4\,y_6] \quad (1.2)$$

```
> cs := [op(cs0), y[5] = 1/4 Q, y[6] = 1/4 Q1, d_x = varpi, ];
     # updating cross-section to include invariantization of y_5, y_6, dx
```

$$cs := \left[x = 0, y_0 = 0, y_1 = 0, y_2 = 0, y_3 = 1, y_4 = 0, y_5 = \frac{Q}{4}, y_6 = \frac{Q1}{4}, d\_x = \varpi\right] \quad (1.3)$$

**Step 1: Defining horizontal and vertical derivative, horizontal and vertical component of a one-form on J^infinity, as well as iota composed with dV and vertpart.**

```
> horpart := eta → Hook(totalD, eta) · d_x :
     # horizontal part of a one-form (NB: d_x is a symbol!)
  vertpart := eta→ add(Hook(D_y[i], eta) · theta || i, i = 0 ..12) : # vertical part of a one-form
  dH := f→ Hook(totalD, ExteriorDerivative(f) ) · d_x : # horizontal derivative of a function
  dV := f→ vertpart(VerticalExteriorDerivative(f) ) : # vertical derivative of a function
  iotavertpart := eta→ add(eval(Hook(D_y[i], eta), cs) · iota_theta || i, i = 0 ..12) :
     # iota composed with vertical part of one-form
  iotadV := f→ add(eval(Hook(D_y[i], ExteriorDerivative(f), cs) · iota_theta || i), i = 0 ..10) :
     # iota composed with dV
```

**Step 2: Computing gamma and epsilon terms**

```
> csvars := map(lhs, cs0) : # list of variables that are constant on cross-section
> for j from 1 to r do;
  gam || j := eval(dH(csvars[j]) + add(LieDerivative(g[i], csvars[j]) · gamma[i], i = 1 ..r),
     cs) : #
  end do:
  gammas := solve([seq(gam || j = 0, j = 1 ..r)], [seq(gamma[j], j = 1 ..r)])[1]
```

$$gammas := \left[\gamma_1 = -\varpi, \gamma_2 = 0, \gamma_3 = 0, \gamma_4 = 0, \gamma_5 = -\frac{Q\,\varpi}{8}, \gamma_6 = -\varpi\right] \quad (1.4)$$

```
> for j from 1 to r do;
  eps || j := iotadV(csvars[j]) + eval(add(LieDerivative(g[i], csvars[j]· epsilon[i]), i = 1 ..r),
     cs) :
```

end do:
epsilons := solve([seq(eps || j = 0, j = 1 ..r)], [seq(epsilon[j], j = 1 ..r)])[1]

$$epsilons := \left[\epsilon_1 = 0, \epsilon_2 = -iota\_theta0, \epsilon_3 = -iota\_theta1, \epsilon_4 = \frac{iota\_theta3}{2}, \epsilon_5 = -\frac{iota\_theta4}{2}, \epsilon_6 = -iota\_theta2\right] \quad (1.5)$$

**Step 3: Computing invariant vertical derivative of Moebius curvature q:**

> dvq := eval(iotadV(q) + eval(add(LieDerivative(g[i], q) · epsilon[i], i = 1 ..r), epsilons), cs)

$$dvq := -2\, Q\, iota\_theta3 - 40\, iota\_theta1 + 4\, iota\_theta5 \quad (1.6)$$

> dvqsigma := eval(iotadV(q1) + eval(add(LieDerivative(g[i], q1) · epsilon[i], i = 1 ..r), epsilons), cs)

$$dvqsigma := -200\, iota\_theta2 - \frac{5\, Q1\, iota\_theta3}{2} - \frac{9\, Q\, iota\_theta4}{2} + 4\, iota\_theta6 \quad (1.7)$$

**Computing invariant vertical derivative of ϖ:**
Here we actually compute the invariant contact form B where d_V(varpi) = B wedge varpi. (Substituting varpi = 1 amounts to hooking with invariant derivation D_sigma. Note minus sign.)

> B := eval(eval(eval(add(epsilon[ i] · horpart( LieDerivative(g[i], dx)) − gamma[i] · iotavertpart(LieDerivative(g[i], dx)), i = 1 ..r), [op(epsilons), op(gammas)]), cs), [varpi = 1])

$$B := \frac{iota\_theta3}{2} \quad (1.8)$$

**Steps 4-5: Computing the correction terms in ι(θ_i+1) = D_omega(ι(θ_i)) + corrterm_i+1.**

> sub := [Q = Q[0], Q1 = Q[1], seq(iota_theta || i = IC || i[0], i = 0 ..6)]

$$sub := \left[Q = Q_0, Q1 = Q_1, iota\_theta0 = IC0_0, iota\_theta1 = IC1_0, iota\_theta2 = IC2_0, iota\_theta3 = IC3_0, iota\_theta4 = IC4_0, iota\_theta5 = IC5_0, iota\_theta6 = IC6_0\right] \quad (1.2.1)$$

Computing the correction terms and written in terms of Q[i] and invariant contact forms IC||i[0]:

> **for** j **from** 1 **to** 6 **do**;
corrterm || j := eval(eval(eval(eval(horpart(add(gamma[i] LieDerivative(g[i], contact_forms[j]), i = 1 ..r)) + add(Hook(D_y[l], (add(gamma[i] LieDerivative(g[i], contact_forms[j]), i = 1 ..r)))·iota_theta || l, l = 0 ..10), [op(epsilons), op(gammas)]), cs), [varpi = 1]), sub);
**end do**:

> DGsetup([s], [Q, seq(IC || i, i = 0 ..5), f], G, 5) :

We express invariant contact forms IC||i[0] in terms of a IC0[0], ICO[1], etc (i.e., as a differential operator acting on IC0[0])

> eq1 := IC1[0] = IC0[1] − corrterm1 : eq := [eq1] :
**for** i **from** 2 **to** 6 **do**: j := i − 1 :
eq || i := IC || i[0] = eval(TotalDiff(eval(IC || j[0], eq), 1) −corrterm || i, eq) ; eq := [op(eq), eq || i] :
**end do**:

> eq5 # example: iota(theta_5) in terms of iota(theta_0) and its derivatives wrt D_sigma

$$IC5_0 = \left(-\frac{Q_2}{8} + 2\right) IC0_1 - \frac{5\, Q_1\, IC0_2}{8} - \frac{Q_0\, IC0_3}{4} + IC0_5 - \frac{3\, IC0_1\, Q_2}{8} - \frac{IC0_0\, Q_3}{8} + 12\, IC0_1 + \frac{Q_0 \left(-\frac{Q_0\, IC0_1}{4} + IC0_3 - \frac{IC0_0\, Q_1}{8}\right)}{4} \tag{1.2.2}$$

**Step 6: Collecting differential operators from dvq, B, Bglobal: (We use the notation that IC||i[j] = D_sigma^j(ι(θ_i)))**

> $DGsetup([s], [Q, seq(IC\|i, i = 0..6), f], G, 5):$

> $dvqnew := expand(eval(eval(dvq, sub), eq));$
$Bnew := expand(eval(eval(B, sub), eq))$

$$dvqnew := \frac{1}{4} Q_0^2\, IC0_1 - 2\, Q_0\, IC0_3 + \frac{1}{8} Q_0\, IC0_0\, Q_1 + 16\, IC0_1 - 2\, IC0_1\, Q_2 - \frac{5}{2} Q_1\, IC0_2 + 4\, IC0_5 - \frac{1}{2} IC0_0\, Q_3$$

$$Bnew := -\frac{Q_0\, IC0_1}{8} + \frac{IC0_3}{2} - \frac{IC0_0\, Q_1}{16} \tag{1.9}$$

> $dvqsigmanew := expand(eval(eval(dvqsigma, sub), eq)):$
$Bglobal := expand\left(Bnew - \frac{dvqsigmanew}{Q[1]}\right):$

**Collecting differential operators:**

> **for** $i$ **from** 0 **to** 5 **do** $A\|i := coeff(dvqnew, IC0[i])$ **end do**: $simplify(dvqnew - add(A\|i\ IC0[i], i = 0..5));$
**for** $i$ **from** 0 **to** 5 **do** $B\|i := coeff(Bnew, IC0[i])$ **end do**: $simplify(Bnew - add(B\|i\ IC0[i], i = 0..5));$
**for** $i$ **from** 0 **to** 6 **do**: $Bglobal\|i := coeff(Bglobal, IC0[i])$ **end do**: $simplify(Bglobal - add(Bglobal\|i\ IC0[i], i = 0..6))$

$$0$$

$$0$$

$$0 \tag{1.10}$$

> $A := collect(expand(add(A\|j\ TotalDiff(IC0[0], [j]), j = 0..5)), [seq(IC0[i], i = 0..5)]):$
$B := collect(expand(add(B\|j\ TotalDiff(IC0[0], [j]), j = 0..5)), [seq(IC0[i], i = 0..5)]):$
$globalB := collect(expand(add(Bglobal\|j\ TotalDiff(IC0[0], [j]), j = 0..6)), [seq(IC0[i], i = 0..6)]):$ *# used for B wrt global invariant coframe*

**Step 7: Computing formal adjoints**

> $Astar := collect(expand(add(TotalDiff((-1)^j\ A\|j \cdot f[0], [j]), j = 0..5)), [f[5], f[4], f[3], f[2], f[1], f[0]]);$
$Bstar := collect(expand(add(TotalDiff((-1)^j\ B\|j \cdot f[0], [j]), j = 0..5)), [f[5], f[4], f[3], f[2], f[1], f[0]])$

$$Astar := -4 f_5 + 2 Q_0 f_3 + \frac{7 Q_1 f_2}{2} + \left(-\frac{Q_0^2}{4} - 16 + 3 Q_2\right) f_1 + \left(-\frac{3 Q_0 Q_1}{8} + Q_3\right) f_0$$

$$Bstar := \frac{Q_1 f_0}{16} + \frac{Q_0 f_1}{8} - \frac{f_3}{2} \qquad (1.11)$$

## Computing examples of projectively invariant EL equations:

**We substitute the Eulerian into Astar, and the Hamiltonian into Bstar.**

> $DGsetup([s], [Q, seq(IC \| i, i = 0..6), f], G, 5):$

Lagrangian = sigma, Eulerian = 0, Hamiltonian = -1

> $EL0 := eval(Bstar, [f[0] = 1, seq(f[l] = 0, l = 1..5)]) = 0;$

$$EL0 := \frac{Q_1}{16} = 0 \qquad (1.12)$$

Lagrangian = q sigma, Eulerian = 1, Hamiltonian = -q

> $EL1 := solve(simplify(eval(Astar, [f[0] = 1, seq(f[l] = 0, l = 1..5)]) + eval(Bstar, [seq(f[l] = Q[l], l = 0..5)])), [Q[3]])[1, 1]$

$$EL1 := Q_3 = \frac{3 Q_0 Q_1}{8} \qquad (1.13)$$

Lagrangian = q^2 sigma, Eulerian = 2q, Hamiltonian = -q^2

> $EL2 := solve(simplify(eval(Astar, [seq(f[l] = TotalDiff(2 Q[0], [l]), l = 0..5)]) + eval(Bstar, [seq(f[l] = TotalDiff(Q[0]^2, [l]), l = 0..5)])), [Q[5]])[1, 1]$

$$EL2 := Q_5 = -\frac{15}{128} Q_1 Q_0^2 + \frac{5}{4} Q_1 Q_2 - 4 Q_1 + \frac{5}{8} Q_0 Q_3 \qquad (1.14)$$

Lagrangian = q^3 sigma, Eulerian = 3q^2, Hamiltonian = -q^3

> $EL2 := solve(simplify(eval(Astar, [seq(f[l] = TotalDiff(3 Q[0]^2, [l]), l = 0..5)]) + eval(Bstar, [seq(f[l] = TotalDiff(Q[0]^3, [l]), l = 0..5)])), [Q[5]])[1, 1]$

$$EL2 := Q_5 = -\frac{1}{384 Q_0} \left(35 Q_1 Q_0^3 - 216 Q_0^2 Q_3 - 1056 Q_0 Q_1 Q_2 - 288 Q_1^3 + 1536 Q_0 Q_1 + 1920 Q_4 Q_1 + 3840 Q_3 Q_2\right) \qquad (1.15)$$

# Computing W:

**Here vt is the invariant contact form of order 0 constructed from the symbol of the Moebius curvature q.**

> $DGsetup([x], [y], E, 12) : \mathrm{omega} := evalDG\left(\frac{1}{\mathrm{sigma}(x)} dx\right):$
>
> $vt := evalDG\left(simplify\left(\frac{1}{4\ \mathrm{sigma}(x)^5}, symbolic\right) (diff(q, y[5]) \cdot (dy[0] - y[1]\, dx))\right);$
>
> $seq(simplify(LieDerivative(g[i], vt), symbolic), i = 1..6)$

$$vt := -\frac{\sqrt{y_1^2 y_3 - 3 y_2^2 y_1 + y_3}\ y_1\, dx}{\left(y_1^2 + 1\right)^2} + \frac{\sqrt{y_1^2 y_3 - 3 y_2^2 y_1 + y_3}\ dy_0}{\left(y_1^2 + 1\right)^2}$$

$$0\, dx, 0\, dx, 0\, dx, 0\, dx, 0\, dx, 0\, dx \qquad (1.3.1)$$

> $W\_moebius := rhs(solve(simplify(DGinfo(evalDG(vt \&w \text{ omega} - W\cdot(dy[0]-y[1]\,dx)$
$\&w\ dx), \text{"CoefficientSet"}), symbolic), [W])[1, 1])$

$$W\_moebius := \frac{y_1^2\, y_3 - 3\, y_2^2\, y_1 + y_3}{\left(y_1^2 + 1\right)^3} \quad \textbf{(1.3.2)}$$

> $solve(W\_moebius, [y[3]])[1]$

$$\left[y_3 = \frac{3\, y_2^2\, y_1}{y_1^2 + 1}\right] \quad \textbf{(1.3.3)}$$

The equation W = 0 describes (unparametrized) circles. We conclude that singular extremals for the Moebius group are precisely the circles.

# Invariant EL using global invariants:

> $DGsetup([x], [y], E, 12):$

> $vartheta\_expr := evalDG\left(\frac{1}{4\ nabla(x)^5}\ (diff(q, y[5])\cdot(dy[0] - y[1]\,dx))\right):$
# global invariant contact form of order 0 constructed from symbol of q and nabla.

> $seq(simplify(LieDerivative(g[i], vartheta\_expr), symbolic), i = 1..6)$

$$0\ dx,\ 0\ dx,\ 0\ dx,\ 0\ dx,\ 0\ dx,\ 0\ dx \quad \textbf{(1.4.1)}$$

**Notation:** Q[0] = q, Q[i] = Dsigma^i(q), Qn[0] = q, Qn[i] = nabla^i(q), IC0 = iota(theta_0)

> $DGsetup([s], [Q, Qn, IC0, \text{vartheta}, f], H):$

> $Nabla := f \to Q[1]\cdot\ TotalDiff(f, [1])$ # TotalDiff is wrt Dsigma

$$\nabla := f \mapsto Q_1 \cdot TotalDiff(f, [1]) \quad \textbf{(1.4.2)}$$

> $Dsig := f \to \text{sqrt}(Qn[1])^{-1}\cdot\ TotalDiff(f, [1])$ # TotalDiff is wrt nabla

$$Dsig := f \mapsto \frac{TotalDiff(f, [1])}{\sqrt{Qn_1}} \quad \textbf{(1.4.3)}$$

**We relate sigma-derivatives of q to nabla-derivatives of q:**

> $sigmatonabla\_q := [Q[0] = Qn[0]]:$
**for** $i$ **from** 1 **to** 7 **do**:
$sigmatonabla\_q := simplify([op(sigmatonabla\_q), Q[i] = Dsig(rhs(sigmatonabla\_q[-1]))],$
$symbolic):$
**end do**: $sigmatonabla\_q[1..3]$

$$\left[Q_0 = Qn_0,\ Q_1 = \sqrt{Qn_1},\ Q_2 = \frac{Qn_2}{2\ Qn_1}\right] \quad \textbf{(1.4.4)}$$

> $nablatosigma\_q := [Qn[0] = Q[0]]:$
**for** $i$ **from** 1 **to** 7 **do**:
$nablatosigma\_q := simplify([op(nablatosigma\_q), Qn[i] = Nabla(rhs(nablatosigma\_q[$
$-1]))], symbolic):$
**end do**: $nablatosigma\_q[1..3]$

$$\left[Qn_0 = Q_0,\ Qn_1 = Q_1^2,\ Qn_2 = 2\ Q_1^2\ Q_2\right] \quad \textbf{(1.4.5)}$$

**We relate invariant contact forms D_sigma^i(iota(theta_0)) to nabla and q.**

```
> sigmatonabla_contact := [IC0[0] = Qn[1]^(5/2) vartheta[0]]:
  for i from 1 to 7 do:
  sigmatonabla_contact := simplify([op(sigmatonabla_contact), IC0[i]
     = Dsig(rhs(sigmatonabla_contact[-1]))], symbolic):
  end do: sigmatonabla_contact[1..3]
```

$$\left[IC0_0 = Qn_1^{5/2}\,\vartheta_0,\ IC0_1 = \vartheta_1\,Qn_1^2 + \frac{5}{2}\,\vartheta_0\,Qn_2\,Qn_1,\ IC0_2 = \frac{2\,Qn_1^2\,\vartheta_2 + 9\,Qn_2\,Qn_1\,\vartheta_1 + 5\,\vartheta_0\,Qn_1\,Qn_3 + 5\,\vartheta_0\,Qn_2^2}{2\,\sqrt{Qn_1}}\right] \tag{1.4.6}$$

**We compute expressions for A, B in terms of global invariants:**

```
> Aglobal := collect(expand(simplify(eval(A, [op(sigmatonabla_q),
     op(sigmatonabla_contact)]), symbolic)), [seq(vartheta[i], i = 0..5)], 'distributed'):
  Bglobal := collect(expand(simplify(eval(globalB, [op(sigmatonabla_q),
     op(sigmatonabla_contact)]), symbolic)), [seq(vartheta[i], i = 0..6)], 'distributed'):
```

**We compute their formal adjoints:**

```
> for i from 0 to 5 do Agl||i := coeff(Aglobal, vartheta[i]) end do:
> simplify(Aglobal - add(Agl||i vartheta[i], i = 0..5))
```

$$0 \tag{1.4.7}$$

```
> for i from 0 to 6 do Bgl||i := coeff(Bglobal, vartheta[i]) end do:
> simplify(Bglobal - add(Bgl||i vartheta[i], i = 0..6))
```

$$0 \tag{1.4.8}$$

```
> Aglobalstar := collect(expand( add( TotalDiff( (-1)^j Agl||j ·f[0] , [j]) ,j = 0..5)),
     [f[5], f[4], f[3], f[2], f[1], f[0]])
```

$$Aglobalstar := -4\,f_5 + \frac{30\,Qn_2\,f_4}{Qn_1} + \left(-\frac{125\,Qn_2^2}{Qn_1^2} + \frac{40\,Qn_3}{Qn_1} + 2\,Qn_1\,Qn_0\right) f_3 + \left(-\frac{255\,Qn_2\,Qn_3}{Qn_1^2} + \frac{7\,Qn_1^2}{2} - 6\,Qn_0\,Qn_2 + \frac{30\,Qn_4}{Qn_1} + \frac{675\,Qn_2^3}{2\,Qn_1^3}\right) f_2 + \left(\frac{1403\,Qn_2^2\,Qn_3}{2\,Qn_1^3} + \frac{19\,Qn_0\,Qn_2^2}{2\,Qn_1} - \frac{129\,Qn_2\,Qn_4}{Qn_1^2} - 16\,Qn_1^2 + \frac{12\,Qn_5}{Qn_1} - \frac{15\,Qn_2\,Qn_1}{4} - \frac{565\,Qn_2^4}{Qn_1^4} - 4\,Qn_0\,Qn_3 - \frac{88\,Qn_3^2}{Qn_1^2} - \frac{Qn_1^2\,Qn_0^2}{4}\right) f_1 + \left(\frac{Qn_1\,Qn_0^2\,Qn_2}{8} + \frac{493\,Qn_2\,Qn_3^2}{2\,Qn_1^3} - \frac{7\,Qn_0\,Qn_2^3}{Qn_1^2} - \frac{797\,Qn_2^3\,Qn_3}{Qn_1^4} + \frac{359\,Qn_2^2\,Qn_4}{2\,Qn_1^3} - \frac{45\,Qn_3\,Qn_4}{Qn_1^2} + \frac{13\,Qn_0\,Qn_2\,Qn_3}{2\,Qn_1} + 8\,Qn_2\,Qn_1 + \frac{2\,Qn_6}{Qn_1} - \frac{26\,Qn_2\,Qn_5}{Qn_1^2} - Qn_0\,Qn_4 - \frac{5\,Qn_3\,Qn_1}{4} - \frac{3\,Qn_0\,Qn_1^3}{8}\right. \tag{1.4.9}$$

$$+\frac{9\,Qn_2^2}{4}+\frac{455\,Qn_2^5}{Qn_1^5}\Bigg)f_0$$

> $Bglobalstar := collect(expand(add(TotalDiff((-1)^j\ Bgl\|j\cdot f[0]\quad,[j])\quad,j=0..6)),$
> $[f[6],f[5],f[4],f[3],f[2],f[1],f[0]])$

$$Bglobalstar := -\frac{4\,f_6}{Qn_1}+\frac{54\,Qn_2\,f_5}{Qn_1^2}+\left(2\,Qn_0-\frac{395\,Qn_2^2}{Qn_1^3}+\frac{100\,Qn_3}{Qn_1^2}\right)f_4+\Bigg(\frac{5\,Qn_1}{2} \qquad (1.4.10)$$

$$-\frac{14\,Qn_0\,Qn_2}{Qn_1}+\frac{110\,Qn_4}{Qn_1^2}-\frac{1195\,Qn_2\,Qn_3}{Qn_1^3}+\frac{3835\,Qn_2^3}{2\,Qn_1^4}\Bigg)f_3+\Bigg(-\frac{Qn_0^2\,Qn_1}{4}$$

$$-\frac{16\,Qn_0\,Qn_3}{Qn_1}+\frac{103\,Qn_0\,Qn_2^2}{2\,Qn_1^2}+\frac{72\,Qn_5}{Qn_1^2}+\frac{13313\,Qn_2^2\,Qn_3}{2\,Qn_1^4}-\frac{999\,Qn_2\,Qn_4}{Qn_1^3}$$

$$-\frac{45\,Qn_2}{4}-\frac{12635\,Qn_2^4}{2\,Qn_1^5}-16\,Qn_1-\frac{688\,Qn_3^2}{Qn_1^3}\Bigg)f_2+\Bigg(-\frac{39\,Qn_3}{4}+40\,Qn_2$$

$$+\frac{26\,Qn_6}{Qn_1^2}-\frac{39725\,Qn_2^3\,Qn_3}{2\,Qn_1^5}+\frac{7515\,Qn_2^2\,Qn_4}{2\,Qn_1^4}+\frac{10415\,Qn_2\,Qn_3^2}{2\,Qn_1^4}-\frac{440\,Qn_2\,Qn_5}{Qn_1^3}$$

$$-\frac{775\,Qn_3\,Qn_4}{Qn_1^3}-\frac{9\,Qn_0\,Qn_4}{Qn_1}-\frac{110\,Qn_0\,Qn_2^3}{Qn_1^3}+\frac{13090\,Qn_2^5}{Qn_1^6}+\frac{5\,Qn_0^2\,Qn_2}{8}$$

$$-\frac{Qn_1^2\,Qn_0}{8}+\frac{26\,Qn_2^2}{Qn_1}+\frac{161\,Qn_0\,Qn_2\,Qn_3}{2\,Qn_1^2}\Bigg)f_1+\Bigg(-3\,Qn_4-\frac{40\,Qn_2^2}{Qn_1}-\frac{109\,Qn_2^3}{4\,Qn_1^2}$$

$$+\frac{4\,Qn_7}{Qn_1^2}-\frac{110\,Qn_4^2}{Qn_1^3}+\frac{688\,Qn_3^3}{Qn_1^4}-\frac{13090\,Qn_2^6}{Qn_1^7}+\frac{Qn_0^2\,Qn_3}{4}+16\,Qn_3+\frac{Qn_1^3}{8}$$

$$-\frac{5675\,Qn_2^3\,Qn_4}{Qn_1^5}-\frac{11864\,Qn_2^2\,Qn_3^2}{Qn_1^5}+\frac{26180\,Qn_2^4\,Qn_3}{Qn_1^6}+\frac{23\,Qn_0\,Qn_2\,Qn_4}{Qn_1^2}$$

$$-\frac{132\,Qn_0\,Qn_2^2\,Qn_3}{Qn_1^3}+\frac{2969\,Qn_2\,Qn_3\,Qn_4}{Qn_1^4}-\frac{5\,Qn_0^2\,Qn_2^2}{8\,Qn_1}+\frac{Qn_1\,Qn_0\,Qn_2}{4}$$

$$-\frac{2\,Qn_0\,Qn_5}{Qn_1}+\frac{16\,Qn_0\,Qn_3^2}{Qn_1^2}+\frac{110\,Qn_0\,Qn_2^4}{Qn_1^4}+\frac{91\,Qn_2\,Qn_3}{4\,Qn_1}-\frac{80\,Qn_2\,Qn_6}{Qn_1^3}$$

$$-\frac{172\,Qn_3\,Qn_5}{Qn_1^3}+\frac{835\,Qn_2^2\,Qn_5}{Qn_1^4}\Bigg)f_0$$

**Example:**

Lagrangian = varpi_2 = q_sigma^-1 sigma

> $EL5 := eval(Bglobalstar,[f[0]=1, seq(f[i]=0, i=1..6)]):$

Converting to q, D_sigma invariants now which we verify against the coordinate expression in the next section

> $eval(EL5, nablatosigma\_q) : solve(simplify(eval(EL5, nablatosigma\_q), symbolic),$
> $[Q[7]])[1]$

$$\left[Q_7 = \frac{1}{64\, Q_1^5} \left(-4\, Q_0^2\, Q_1^5\, Q_3 + 12\, Q_1^4\, Q_0^2\, Q_2^2 - 4\, Q_1^6\, Q_0\, Q_2 - Q_1^8 + 32\, Q_0\, Q_1^5\, Q_5 - 384\, Q_0\, Q_1^4\, Q_2\, Q_4 - 288\, Q_0\, Q_1^4\, Q_3^2 + 2304\, Q_0\, Q_1^3\, Q_2^2\, Q_3 - 1920\, Q_0\, Q_2^4\, Q_1^2 + 48\, Q_1^6\, Q_4 - 392\, Q_1^5\, Q_2\, Q_3 + 480\, Q_1^4\, Q_2^3 - 256\, Q_1^5\, Q_3 + 768\, Q_1^4\, Q_2^2 + 1152\, Q_1^4\, Q_2\, Q_6 + 2880\, Q_1^4\, Q_3\, Q_5 + 1920\, Q_1^4\, Q_4^2 - 11520\, Q_1^3\, Q_2^2\, Q_5 - 46080\, Q_1^3\, Q_2\, Q_3\, Q_4 - 11520\, Q_1^3\, Q_3^3 + 76800\, Q_1^2\, Q_2^3\, Q_4 + 172800\, Q_1^2\, Q_2^2\, Q_3^2 - 345600\, Q_1\, Q_2^4\, Q_3 + 161280\, Q_2^6\right)\right] \quad \textbf{(1.4.11)}$$

# Verifying invariant EL examples using coordinate expressions:

> $\#DGsetup([x], [y], E, 12) :$

> $\#slj := solve\left(\{seq(q \| k = Q \| k, k = 0..7)\}, \left\{seq\left(y_k, k = 5..12\right)\right\}\right) :$

> $\#slj0 := \left\{x = 0, y_0 = 0, y_1 = 0, y_2 = 0, y_3 = 1, y_4 = 0\right\} : slj0 := slj0$ **union** $factor(simplify(eval(slj, slj0), symbolic)) :$

> $\#L1 := simplify\left(\sqrt{\kappa 1}\,\sqrt{1 + y_1^2}, symbolic\right); L2 := simplify\left(q\sqrt{\kappa 1}\,\sqrt{1 + y_1^2}, symbolic\right);$
> $L3 := simplify\left(q^2\sqrt{\kappa 1}\,\sqrt{1 + y_1^2}, symbolic\right); L4 := simplify\left(q^3\sqrt{\kappa 1}\,\sqrt{1 + y_1^2}, symbolic\right) : L5 := simplify\left(\frac{1}{q1}\sqrt{\kappa 1}\,\sqrt{1 + y_1^2}, symbolic\right) :$

$$L1 := \frac{\sqrt{y_1^2\, y_3 - 3\, y_2^2\, y_1 + y_3}}{y_1^2 + 1}$$

$$L2 := \frac{1}{\left(y_1^2\, y_3 - 3\, y_2^2\, y_1 + y_3\right)^{5/2}\left(y_1^2 + 1\right)}\left(\left(135\, y_1^4 - 270\, y_1^2 - 45\right) y_2^6 + \left(-180\, y_1^5 + 180\, y_1\right) y_3\, y_2^4 + 30\, y_4\left(y_1^2 + 1\right)^3 y_2^3 - 12\left(y_1^2 + 1\right)^2\left(\left(\left(-\frac{10\, y_1^2}{3} + \frac{20}{3}\right) y_3^2 + y_1\, y_5\left(y_1^2 + 1\right)\right) y_2^2 + 40\, y_1\, y_3\, y_4\left(y_1^2 + 1\right)^3 y_2 + 4\left(y_1^2 + 1\right)^3\left(-10\, y_1\, y_3^3 + y_5\left(y_1^2 + 1\right) y_3 - \frac{5\, y_4^2\left(y_1^2 + 1\right)}{4}\right)\right)$$

$$L3 := \frac{1}{\left(y_1^2\, y_3 - 3\, y_2^2\, y_1 + y_3\right)^{11/2}\left(y_1^2 + 1\right)}\left(16\left(\left(\frac{135}{4}\, y_1^4 - \frac{135}{2}\, y_1^2 - \frac{45}{4}\right) y_2^6 + \left(-45\, y_1^5 + 45\, y_1\right) y_3\, y_2^4 + \frac{15\, y_4\left(y_1^2 + 1\right)^3 y_2^3}{2} - 3\left(y_1^2 + 1\right)^2\left(\left(-\frac{10\, y_1^2}{3} + \frac{20}{3}\right) y_3^2 + y_1\, y_5\left(y_1^2\right.\right.\right.\right. \quad \textbf{(1.5.1)}$$

$$+1)\Big) y_2^2 + 10\, y_1\, y_3\, y_4 \left(y_1^2+1\right)^3 y_2 + \left(y_1^2+1\right)^3 \Big(-10\, y_1\, y_3^3 + y_5 \left(y_1^2+1\right) y_3 - \frac{5\, y_4^2 \left(y_1^2+1\right)}{4}\Big)\Big)\Big)^2\Big)$$

Lagrangian = sigma

> #EL1:=EulerLagrange(L1) : EL1 := eval(EL1, slj0) : length(EL1); evalf(log[10](%)); EL1 := factor(simplify(EL1, symbolic));

$$15$$

$$1.176091259$$

$$EL1 := \left[\frac{Q1}{16}\right] \quad \textbf{(1.5.2)}$$

Lagrangian = q sigma

> #EL2:=EulerLagrange(L2) : EL2 := eval(EL2, slj0) : length(EL2); evalf(log[10](%)); EL2 := factor(simplify(EL2, symbolic)) : solve(EL2, {Q3})

$$33$$

$$1.518513940$$

$$\left\{Q3 = \frac{3\, Q0\, Q1}{8}\right\} \quad \textbf{(1.5.3)}$$

Lagrangian = q^2 sigma

> #EL3:=EulerLagrange(L3) : length(EL3); evalf(log[10](%)); EL3 := eval(EL3, slj0) : length(EL3); evalf(log[10](%)); EL3 := factor(simplify(EL3, symbolic)) : solve(EL3, {Q5})

$$169695523$$

$$8.229670386$$

$$360$$

$$2.556302501$$

$$\left\{Q5 = -4\, Q1 - \frac{15}{128}\, Q0^2\, Q1 + \frac{5}{8}\, Q0\, Q3 + \frac{5}{4}\, Q1\, Q2\right\} \quad \textbf{(1.5.4)}$$

Lagrangian = q^3 sigma

> #EL4:=EulerLagrange(L4) : EL4 := eval(EL4, slj0) : length(EL4); evalf(log[10](%)); solve(factor(simplify(EL4, symbolic)), [Q5])[1]

$$1275$$

$$3.105510185$$

$$\Big[Q5 = -\frac{1}{384\, Q0}\big(35\, Q0^3\, Q1 - 216\, Q0^2\, Q3 - 1056\, Q0\, Q1\, Q2 - 288\, Q1^3 + 1536\, Q0\, Q1 + 1920\, Q1\, Q4 + 3840\, Q2\, Q3\big)\Big] \quad \textbf{(1.5.5)}$$

>

Lagrangian = Delta = q_sigma^-1 sigma

> #EL5:=EulerLagrange(L5) : EL5 := eval(EL5, slj0) : length(EL5); evalf(log[10](%));

$simplify(solve(factor(simplify(EL5, symbolic)), [Q7])[1], symbolic)$

>

# Projective 2D

> $restart : with(DifferentialGeometry) : with(LieAlgebras) : with(Tensor) : with(GroupActions) :$
> $with(Tools) : Preferences(\text{"ShowFramePrompt"},'false') : interface(warnlevel = 0) :$
> $with(LinearAlgebra) : with(PDETools) : with(JetCalculus) : with(ArrayTools) :$
> $Preferences(\text{"JetNotation"}, \text{"JetNotation2"}) :$

>

> $DGsetup([x], [y], E, 12) : totalD := evalDG(D\_x + add(y[i+1]\ D\_y[i], i = 0..10)) :$
> $contact\_forms := [seq(dy[i] - y[i+1]\, dx, i = 0..8)] :$

**Lie algebra of projective group:**

> $proj := evalDG([D\_x, D\_y[0], x\, D\_x, x\, D\_y[0], y[0]\, D\_x, y[0]\, D\_y[0], x^2\, D\_x + x\, y[0]\, D\_y[0], x\, y[0]\, D\_x + y[0]^2\, D\_y[0]]) : g := map(Prolong, proj, 10) : r := nops(proj) :$

**Relative invariants and absolute invariants:**

> $R_{2,1} := y_2 : R_{9,3} := 9\, y_2^2\, y_5 - 45\, y_2\, y_3\, y_4 + 40\, y_3^3 : S_{3,0} := \frac{R_{9,3}}{R_{2,1}^3} : S_{8,0} :=$
> $simplify\left(6\, S_{3,0}\, TotalDiff(S_{3,0}, [2]) - 7\, TotalDiff(S_{3,0}, [1])^2 + 27\, S_{3,0}^2\, R_{2,1}^{\frac{1}{3}} TotalDiff\left(R_{2,1}^{-\frac{1}{3}}, [2]\right), symbolic\right) : R_{24,8} := simplify\left(R_{2,1}^8\, S_{8,0}, symbolic\right) :$
> $\text{kappa} := \frac{R_{24,8}}{R_{9,3}^{\frac{8}{3}}} : Dp := f \rightarrow \left(9^{\frac{1}{3}}\ S_{3,0}^{-\frac{1}{3}}\ TotalDiff(f, [1])\right) :$

> $kappa0 := \text{kappa} :$ **for** $k$ **from** 1 **to** 7 **do** $\text{kappa} \| k := Dp(simplify(\text{kappa} \| (k-1), symbolic))$:
> **od**:

> $seq(simplify(LieDerivative(Prolong(proj[i], 10), [\text{kappa}, kappa1])), i = 1..8)$
> *# checking that kappa and kappa1 are projectively invariant*

$$[0, 0], [0, 0], [0, 0], [0, 0], [0, 0], [0, 0], [0, 0], [0, 0] \quad \textbf{(2.1)}$$

**Cross-section:**

> $cs0 := [x = 0, y[0] = 0, y[1] = 0, y[2] = 1, y[3] = 0, y[4] = 0, y[5] = 1, y[6] = 0] :$
> *# cross-section*
> $invariantizations := solve(\, eval(\text{kappa} = K, cs0), [y[7]])[1]$

$$invariantizations := \left[y_7 = \frac{K\, 9^{2/3}}{6}\right] \quad \textbf{(2.2)}$$

> $cs := [\, op(cs0), op(invariantizations), d\_x = \text{varpi}, \,];$
> *# updating cross-section to include invariantization of y_7, dx*

$$cs := \left[x = 0, y_0 = 0, y_1 = 0, y_2 = 1, y_3 = 0, y_4 = 0, y_5 = 1, y_6 = 0, y_7 = \frac{K\, 9^{2/3}}{6}, d\_x = \varpi\right] \quad \textbf{(2.3)}$$

**Step 1: Defining horizontal and vertical derivative, horizontal and vertical component of a one-**

**form on J^infinity, as well as iota composed with dV and vertpart.**

```
> horpart := eta -> Hook(totalD, eta) · d_x :
      # horizontal part of a one-form (NB: d_x is a symbol!)
  vertpart := eta -> add(Hook(D_y[i], eta) · theta || i, i = 0 ..12) : # vertical part of a one-form
  dH := f -> Hook(totalD, ExteriorDerivative(f) ) · d_x : # horizontal derivative of a function
  dV := f -> vertpart(VerticalExteriorDerivative(f) ) : # vertical derivative of a function
  iotavertpart := eta -> add(eval(Hook(D_y[i], eta), cs) · iota_theta || i, i = 0 ..12) :
      # iota composed with vertical part of one-form
  iotadV := f -> add(eval(Hook(D_y[i], ExteriorDerivative(f), cs) · iota_theta || i), i = 0 ..10) :
      # iota composed with dV
```

**Step 2: Computing gamma and epsilon terms**

```
> csvars := map(lhs, cs0) : # list of variables that are constant on cross-section
> for j from 1 to r do;
  gam || j := eval(dH(csvars[j]) + add(LieDerivative(g[i], csvars[j]) · gamma[i], i = 1 ..r),
      cs) : #
  end do:
  gammas := solve([seq(gam || j = 0, j = 1 ..r)], [seq(gamma[j], j = 1 ..r)])[1]
```

$$gammas := \left[\gamma_1 = -\varpi, \gamma_2 = 0, \gamma_3 = 0, \gamma_4 = -\varpi, \gamma_5 = -\frac{K\, 9^{2/3}\, \varpi}{18}, \gamma_6 = 0, \gamma_7 = \frac{K\, 9^{2/3}\, \varpi}{18}, \gamma_8 = \frac{\varpi}{6}\right] \quad (2.4)$$

```
> for j from 1 to r do;
  eps || j := iotadV(csvars[j]) + eval(add(LieDerivative(g[i], csvars[j]· epsilon[i]), i = 1 ..r),
      cs) :
  end do:
  epsilons := solve([seq(eps || j = 0, j = 1 ..r)],  [seq(epsilon[j], j = 1 ..r )])[1]
```

$$epsilons := \left[\epsilon_1 = 0, \epsilon_2 = -iota\_theta0, \epsilon_3 = \frac{iota\_theta5}{3} - \frac{iota\_theta2}{3}, \epsilon_4 = -iota\_theta1, \epsilon_5 = \frac{8\, iota\_theta3}{3} - \frac{iota\_theta6}{3}, \epsilon_6 = -\frac{5\, iota\_theta2}{3} + \frac{2\, iota\_theta5}{3}, \epsilon_7 = \frac{iota\_theta6}{3} - \frac{7\, iota\_theta3}{3}, \epsilon_8 = \frac{iota\_theta4}{6}\right] \quad (2.5)$$

**Step 3: Computing invariant vertical derivative of projective curvature kappa:**

```
> dvkappa := eval(iotadV(kappa) + eval(add(LieDerivative(g[i], kappa) · epsilon[i], i = 1
      ..r), epsilons), cs)
```

$$dvkappa := \frac{2\, K\, iota\_theta2}{3} - \frac{35\, 9^{1/3}\, iota\_theta4}{3} - \frac{5\, K\, iota\_theta5}{3} + \frac{2\, 9^{1/3}\, iota\_theta7}{3} \quad (2.6)$$

**Computing invariant vertical derivative of $\varpi$:**

```
> B := eval(eval(eval(add(epsilon[ i] · horpart( LieDerivative(g[i], dx))  − gamma[i]
      · eval(iotavertpart(LieDerivative(g[i], dx), [theta0 = iota_theta0])), i = 1 ..r),
      [op(epsilons), op(gammas)]), cs), [varpi = 1])
```

$$B := \frac{iota\_theta5}{3} - \frac{iota\_theta2}{3} + \frac{K\, 9^{2/3}\, iota\_theta0}{18} \quad (2.7)$$

**Steps 4-5: Computing the correction terms in ι(θ_i+1) = Dp(ι(θ_i)) + corrterm_i+1.**

```
> sub := [K = K[0], K1 = K[1], seq(iota_theta || i = IC || i[0], i = 0 ..7) ]
```

$$sub := [K = K_0, K1 = K_1, iota\_theta0 = IC0_0, iota\_theta1 = IC1_0, iota\_theta2 = IC2_0, iota\_theta3 = IC3_0, iota\_theta4 = IC4_0, iota\_theta5 = IC5_0, iota\_theta6 = IC6_0, iota\_theta7 = IC7_0] \quad \textbf{(2.1.1)}$$

```
> for j from 1 to 8 do;
  corrterm || j := eval(eval(eval(eval(horpart(add(gamma[i] LieDerivative(g[i],
      contact_forms[j]), i = 1 ..r) ) + add(Hook(D_y[l], (add(gamma[i] LieDerivative(g[i],
      contact_forms[j]), i = 1 ..r) ) )·iota_theta || l , l = 0 ..10), [op(epsilons), op(gammas)]),
     cs), [varpi = 1]), sub); # substituting varpi=1 amounts to hooking with Dp
  end do:
> DGsetup([s], [K, seq(IC || i, i = 0 ..8), f], G, 5) :
> eq1 := IC1[0] = IC0[1] − corrterm1 : eq := [eq1] :
  for i from 2 to 8 do: j := i − 1 :
  eq || i := IC || i[0] = eval(TotalDiff(eval(IC || j[0], eq), 1) −corrterm || i, eq) ; eq := [op(eq),
      eq || i] :
  end do:
> eq3 # example
```

$$IC3_0 = -\frac{5\,K_0\,9^{2/3}\,IC0_1}{18} + IC0_3 - \frac{9^{2/3}\,IC0_0\,K_1}{9} \quad \textbf{(2.1.2)}$$

**Step 6: Collecting differential operators from dvq, B:**

```
> DGsetup([s], [K, seq(IC || i, i = 0 ..7), f], G, 5) :
> dvkappanew := expand(eval(eval(dvkappa , sub), eq));
  Bnew := expand(eval(eval(B , sub), eq))
```

$$dvkappanew := -\frac{8\,K_0^3\,9^{1/3}\,IC0_1}{27} + \frac{2\,K_0^2\,9^{2/3}\,IC0_3}{3} + \frac{32\,9^{2/3}\,IC0_1\,K_1^2}{27} - \frac{13\,IC0_1\,K_4}{3} - \frac{2\,IC0_0\,K_5}{3} + \frac{2\,9^{1/3}\,IC0_7}{3} - \frac{35\,IC0_2\,K_3}{3} - \frac{49\,IC0_3\,K_2}{3} - \frac{35\,IC0_4\,K_1}{3} + \frac{K_1\,IC0_1}{2} - 4\,K_0\,IC0_5 + \frac{55\,K_0\,IC0_2\,9^{2/3}\,K_1}{27} - \frac{8\,K_1\,K_0^2\,9^{1/3}\,IC0_0}{27} + \frac{10\,K_0\,9^{2/3}\,IC0_0\,K_3}{27} + \frac{8\,9^{2/3}\,K_1\,IC0_0\,K_2}{9} + \frac{41\,K_0\,9^{2/3}\,IC0_1\,K_2}{27} + \frac{9^{1/3}\,IC0_1}{2}$$

$$Bnew := -\frac{9^{2/3}\,IC0_1\,K_2}{6} + \frac{4\,K_0^2\,9^{1/3}\,IC0_1}{27} - \frac{5\,IC0_2\,9^{2/3}\,K_1}{18} + \frac{IC0_2}{2} - \frac{5\,K_0\,9^{2/3}\,IC0_3}{27} + \frac{IC0_5}{3} + \frac{4\,K_1\,K_0\,9^{1/3}\,IC0_0}{27} - \frac{9^{2/3}\,IC0_0\,K_3}{27} \quad \textbf{(2.8)}$$

**Collecting differential operators:**

```
> for i from 0 to 7 do A || i := coeff(dvkappanew, IC0[i]) end do: simplify(dvkappanew
      − add(A || i IC0[i], i = 0 ..7) );
  for i from 0 to 7 do B || i := coeff(Bnew, IC0[i]) end do: simplify(Bnew − add(B || i IC0[i],
      i = 0 ..7) );
```

$$0$$
$$0 \quad \textbf{(2.9)}$$

> $A := collect(expand(add(A||j\ TotalDiff(IC0[0], [j]), j = 0..7)), [seq(IC0[i], i = 0..7)])$ :
> $B := collect(expand(add(B||j\ TotalDiff(IC0[0], [j]), j = 0..5)), [seq(IC0[i], i = 0..5)])$ :

**Step 7: Computing formal adjoints**

> $Astar := collect\big(expand\big(add\big(TotalDiff\big((-1)^j\ A||j \cdot f[0], [j]\big), j = 0..7\big)\big), [seq(f[i], i = 0..7)]\big)$;
> $Bstar := collect\big(expand\big(add\big(TotalDiff\big((-1)^j\ B||j \cdot f[0], [j]\big), j = 0..7\big)\big), [seq(f[i], i = 0..7)]\big)$

$$Astar := \left(-\frac{8\, 9^{2/3} K_1 K_2}{9} + \frac{16 K_1 K_0^2 9^{1/3}}{27} - \frac{4 K_0 9^{2/3} K_3}{9} - \frac{K_2}{2} + \frac{2 K_5}{3}\right) f_0 + \left(-\frac{13 K_0 9^{2/3} K_2}{9} - \frac{9^{1/3}}{2} - \frac{10\, 9^{2/3} K_1^2}{9} + \frac{8 K_0^3 9^{1/3}}{27} - \frac{K_1}{2} + \frac{10 K_4}{3}\right) f_1 + \left(-\frac{53 K_0 9^{2/3} K_1}{27} + \frac{22 K_3}{3}\right) f_2 + \left(\frac{29 K_2}{3} - \frac{2 K_0^2 9^{2/3}}{3}\right) f_3 - \frac{2\, 9^{1/3} f_7}{3} + 4 K_0 f_5 + \frac{25 K_1 f_4}{3}$$

$$Bstar := \left(-\frac{4 K_0 9^{1/3} K_1}{27} + \frac{9^{2/3} K_3}{27}\right) f_0 + \left(\frac{9^{2/3} K_2}{6} - \frac{4 K_0^2 9^{1/3}}{27}\right) f_1 + \left(\frac{5\, 9^{2/3} K_1}{18} + \frac{1}{2}\right) f_2 + \frac{5 K_0 9^{2/3} f_3}{27} - \frac{f_5}{3} \quad \textbf{(2.10)}$$

## Computing examples of projectively-invariant EL equations

> $DGsetup([s], [K, seq(IC||i, i = 0..7), f], G, 5)$ :

Lagrangian = varpi

> $EL0 := solve(simplify(eval(Bstar, [f[0] = 1, seq(f[l] = 0, l = 1..5)]), symbolic) = 0, [K[3]])[1]$;

$$EL0 := \left[K_3 = \frac{4 K_0 3^{1/3} K_1}{3}\right] \quad \textbf{(2.11)}$$

Lagrangian = kappa varpi

> $EL1 := solve(simplify(eval(Astar, [f[0] = 1, seq(f[l] = 0, l = 1..7)]) + eval(Bstar, [seq(f[l] = K[l], l = 0..5)])), [K[5]])[1]$

$$EL1 := \left[K_5 = 4\, 3^{1/3} K_1 K_2 - \frac{8 K_1 K_0^2 3^{2/3}}{9} + 2 K_0 3^{1/3} K_3\right] \quad \textbf{(2.12)}$$

Lagrangian = kappa^2 varpi

> $EL2 := solve\big(simplify\big(eval(Astar, [seq(f[l] = TotalDiff(2 K[0], [l]), l = 0..7)])$

$+ eval(Bstar, [seq(f[l]=TotalDiff(K[0]^2,[l]), l=0..5)])), [K[7]])[1]$

$$EL2 := \left[K_7 = \frac{1}{36}\left(\left(12\,K_1\,K_0^3\,3^{2/3} - 49\,K_0^2\,3^{1/3}\,K_3 - 178\,K_0\,3^{1/3}\,K_1\,K_2 - 45\,3^{1/3}\,K_1^3 - 9\,K_1\,3^{2/3} + 78\,K_0\,K_5 + 180\,K_1\,K_4 + 246\,K_3\,K_2\right)3^{1/3}\right)\right] \quad (2.13)$$

## Verifying invariant EL examples using coordinate expressions:

> #DGsetup ([x], [y], E, 12) :

> #slj:=solve( {seq(kappa || k = K || k, k = 0..7)}, {seq($(y_k$, k = 7..14)}) :

> #slj0:= {x = 0, y[0] = 0, y[1] = 0, y[2] = 1, y[3] = 0, y[4] = 0, y[5] = 1, y[6 ] = 0} : slj0 := slj0 **union** factor(simplify(eval(slj, slj0), symbolic)) :

> #slr:=solve( {$R_{2,1} = r_1$, $R_{9,3} = r_3$}, {$y_5$, $y_2$}) :

> #L1:=simplify$\left(9^{-\frac{1}{3}}\ S_{3,0}^{\frac{1}{3}}\right.$ kappa, symbolic$\left.\right)$; L2 := simplify$\left(9^{-\frac{1}{3}}\ S_{3,0}^{\frac{1}{3}}\,\kappa^2, symbolic\right)$; L3 := simplify$\left(9^{-\frac{1}{3}}\ S_{3,0}^{\frac{1}{3}}\,\kappa^{-1}, symbolic\right)$

$$L1 := \frac{1}{y_2\left(9\,y_2^2\,y_5 - 45\,y_2\,y_3\,y_4 + 40\,y_3^3\right)^{7/3}}\Big(3^{1/3}\big(162\,y_2^6\,y_5\,y_7 - 189\,y_2^6\,y_6^2 - 810\,y_2^5\,y_3\,y_4\,y_7 + 1134\,y_2^5\,y_3\,y_5\,y_6 + 1890\,y_2^5\,y_4^2\,y_6 - 2835\,y_5^2\,y_2^5\,y_4 + 720\,y_2^4\,y_3^3\,y_7 - 3150\,y_2^4\,y_3^2\,y_4\,y_6 - 756\,y_5^2\,y_2^4\,y_3^2 + 13230\,y_5\,y_3\,y_2^4\,y_4^2 - 4725\,y_2^4\,y_4^4 - 12600\,y_5\,y_3^3\,y_2^3\,y_4 - 7875\,y_2^3\,y_3^2\,y_4^3 + 6720\,y_5\,y_3^5\,y_2^2 + 31500\,y_2^2\,y_3^4\,y_4^2 - 33600\,y_2\,y_3^6\,y_4 + 11200\,y_3^8\big)\Big)$$

$$L2 := \frac{1}{y_2\left(9\,y_2^2\,y_5 - 45\,y_2\,y_3\,y_4 + 40\,y_3^3\right)^5}\Big(3\,3^{1/3}\big(162\,y_2^6\,y_5\,y_7 - 189\,y_2^6\,y_6^2 - 810\,y_2^5\,y_3\,y_4\,y_7 + 1134\,y_2^5\,y_3\,y_5\,y_6 + 1890\,y_2^5\,y_4^2\,y_6 - 2835\,y_5^2\,y_2^5\,y_4 + 720\,y_2^4\,y_3^3\,y_7 - 3150\,y_2^4\,y_3^2\,y_4\,y_6 - 756\,y_5^2\,y_2^4\,y_3^2 + 13230\,y_5\,y_3\,y_2^4\,y_4^2 - 4725\,y_2^4\,y_4^4 - 12600\,y_5\,y_3^3\,y_2^3\,y_4 - 7875\,y_2^3\,y_3^2\,y_4^3 + 6720\,y_5\,y_3^5\,y_2^2 + 31500\,y_2^2\,y_3^4\,y_4^2 - 33600\,y_2\,y_3^6\,y_4 + 11200\,y_3^8\big)^2\Big)$$

$$L3 := \left(3^{1/3}\left(9\,y_2^2\,y_5 - 45\,y_2\,y_3\,y_4 + 40\,y_3^3\right)^3\right)\Big/\Big(9\,y_2\big(162\,y_2^6\,y_5\,y_7 - 189\,y_2^6\,y_6^2 - 810\,y_2^5\,y_3\,y_4\,y_7 + 1134\,y_2^5\,y_3\,y_5\,y_6 + 1890\,y_2^5\,y_4^2\,y_6 - 2835\,y_5^2\,y_2^5\,y_4 + 720\,y_2^4\,y_3^3\,y_7 - 3150\,y_2^4\,y_3^2\,y_4\,y_6 - 756\,y_5^2\,y_2^4\,y_3^2 + 13230\,y_5\,y_3\,y_2^4\,y_4^2 - 4725\,y_2^4\,y_4^4 - 12600\,y_5\,y_3^3\,y_2^3\,y_4 - 7875\,y_2^3\,y_3^2\,y_4^3 + 6720\,y_5\,y_3^5\,y_2^2 + 31500\,y_2^2\,y_3^4\,y_4^2 - 33600\,y_2\,y_3^6\,y_4 + 11200\,y_3^8\big)\Big) \quad (2.2.1)$$

Lagrangian = varpi

> #EL0:=factor$\left(simplify\left(eval\left(eval\left(EulerLagrange\left(9^{-\frac{1}{3}}\ S_{3,0}^{\frac{1}{3}}\right), slj\right), slr\right), symbolic\right)\right)$ : solve(EL0, {K3})

$$\left\{K3 = \frac{4\,K0\,K1\,3^{1/3}}{3}\right\} \quad (2.2.2)$$

Lagrangian = kappa varpi

```
> #EL1:=EulerLagrange(L1) : EL1b := simplify(eval(eval(EL1, slj), slr) , symbolic) :
    factor(simplify(EL1b, symbolic)) : solve(%, {K5})
```

Lagrangian = kappa^2 varpi

```
> #EL2:=EulerLagrange(L2) : EL2b := simplify(eval(eval(EL2, slj), slr) , symbolic) :
    factor(simplify(EL2b, symbolic)) : solve(%, {K7})
```

# Euclidean 3D

```
> restart : with(DifferentialGeometry) : with(LieAlgebras) : with(Tensor) : with(GroupActions) :
    with(Tools) : Preferences("ShowFramePrompt",'false') : interface(warnlevel = 0) :
    with(LinearAlgebra) : with(PDETools) : with(JetCalculus) : with(ArrayTools) :
    Preferences("JetNotation", "JetNotation2") :
> DGsetup([x], [y, z], E, 12) : totalD := evalDG(D_x + add(y[i + 1] D_y[i], i = 0..10 )
    + add(z[i + 1] D_z[i], i = 0..10 )) : contact_forms := [seq(op([dy[i] − y[i + 1] dx,
    dz[i] − z[i + 1] dx]), i = 0..8)] :
```

**Lie algebra of Euclidean group:**

```
> iso := evalDG([D_x, D_y[0], D_z[0], x D_y[0] − y[0] D_x, x D_z[0] − z[0] D_x,
    y[0] D_z[0] − z[0] D_y[0]]) : g := map(Prolong, iso, 10) : r := nops(iso) :
```

**Local invariants:**

$$> \text{kappa} := \frac{\text{sqrt}\left((y[1]z[2]-y[2]z[1])^2+y[2]^2+z[2]^2\right)}{\left(1+y[1]^2+z[1]^2\right)^{\frac{3}{2}}};\ \text{tau} := \frac{(y[2]z[3]-z[2]y[3])}{(y[1]z[2]-z[1]y[2])^2+y[2]^2+z[2]^2};$$

$$\kappa := \frac{\sqrt{(y_1 z_2 - z_1 y_2)^2 + y_2^2 + z_2^2}}{\left(y_1^2 + z_1^2 + 1\right)^{3/2}}$$

$$\tau := \frac{y_2 z_3 - z_2 y_3}{(y_1 z_2 - z_1 y_2)^2 + y_2^2 + z_2^2} \qquad \textbf{(3.1)}$$

$$> Ts := f \to simplify\left(\frac{1}{\text{sqrt}\left(1+y[1]^2+z[1]^2\right)} \cdot TotalDiff(f, x),\ symbolic\right):$$

\# *invariant derivation (i.e., wrt arclength)*

$$\kappa 0 := \kappa \text{ :}\textbf{for } i \textbf{ to } 3 \textbf{ do } \kappa \| i := Ts\left(\kappa \| (i-1)\right)\text{:}\textbf{od}\text{:}$$

$$\tau 0 := \tau \text{ :}\textbf{for } i \textbf{ to } 2 \textbf{ do } \tau \| i := Ts\left(\tau \| (i-1)\right)\text{:}\textbf{od}\text{:}$$

```
> seq(simplify(LieDerivative(g[i], [kappa, tau, kappa1, tau1])), i = 1..r)
    # checking that these are invariant
```

[0, 0, 0, 0], [0, 0, 0, 0], [0, 0, 0, 0], [0, 0, 0, 0], [0, 0, 0, 0], [0, 0, 0, 0] **(3.2)**

Defining cross-section:

```
> cs0 := [x = 0, y[0] = 0, z[0] = 0, y[1] = 0, z[1] = 0, z[2] = 0] # Frenet--Serret cross-section
```

$$cs0 := [x=0, y_0=0, z_0=0, y_1=0, z_1=0, z_2=0] \quad (3.3)$$

**Relating invariantization to invariants:**

> simplify(eval([kappa = K, tau = T, kappa1 = K1, tau1 = T1], cs0), symbolic)

$$\left[y_2 = K, \frac{z_3}{y_2} = T, y_3 = K1, \frac{y_2 z_4 - 2 y_3 z_3}{y_2^2} = T1\right] \quad (3.4)$$

> simplify(eval([kappa = K, tau = T, kappa1 = K1], cs0), symbolic) : invariantizations := solve(%, [ y[3], y[2], z[3]])[1]

$$invariantizations := [y_3 = K1, y_2 = K, z_3 = K\,T] \quad (3.5)$$

> cs := [x = 0, y[0] = 0, z[0] = 0, y[1] = 0, z[1] = 0, z[2] = 0, op(invariantizations), d_x = varpi]

$$cs := [x=0, y_0=0, z_0=0, y_1=0, z_1=0, z_2=0, y_3=K1, y_2=K, z_3=K\,T, d\_x=\varpi] \quad (3.6)$$

**Step 1: Defining horizontal and vertical derivative, horizontal and vertical component of a one-form on J^infinity, as well as iota composed with dV and vertpart.**

> horpart := eta → Hook(totalD, eta) · d_x :
    # horizontal part of a one-form (NB: d_x is a symbol!)
  vertpart := eta→ add(Hook(D_y[i], eta) · cat(theta_y, i) + Hook(D_z[i], eta) · cat(theta_z, i),
    i = 0 ..12) : # vertical part of a one-form
  dH := f→ Hook(totalD, ExteriorDerivative(f) ) · d_x : # horizontal derivative of a function
  dV := f→ vertpart(VerticalExteriorDerivative(f) ) : # vertical derivative of a function
  iotavertpart := eta→ add(eval(Hook(D_y[i], eta), cs) · cat(iota_theta_y, i)
    + eval(Hook(D_z[i], eta), cs) · cat(iota_theta_z, i), i = 0 ..12) :
    # iota composed with vertical part of one-form
  iotadV := f→ add(eval(Hook(D_y[i], ExteriorDerivative(f), cs) · cat(iota_theta_y, i)
    + Hook(D_z[i], ExteriorDerivative(f), cs) · cat(iota_theta_z, i) ), i = 0 ..10) :
    # iota composed with dV

**Step 2: Computing gamma and epsilon terms**

> csvars := map(lhs, cs0) : # list of variables that are constant on cross-section

> **for** j **from** 1 **to** r **do**;
  gam || j := eval(dH(csvars[j]) + add(LieDerivative(g[i], csvars[j]) · gamma[i], i = 1 ..r),
    cs) :
  **end do**:
  gammas := solve([seq(gam || j = 0, j = 1 ..r)], [seq(gamma[j], j = 1 ..r)])[1]

$$gammas := [\gamma_1 = -\varpi, \gamma_2 = 0, \gamma_3 = 0, \gamma_4 = -K\,\varpi, \gamma_5 = 0, \gamma_6 = -T\,\varpi] \quad (3.7)$$

> **for** j **from** 1 **to** r **do**;
  eps || j := iotadV(csvars[j]) + eval(add(LieDerivative(g[i], csvars[j] · epsilon[i]), i = 1 ..r),
    cs) :
  **end do**:
  epsilons := solve([seq(eps || j = 0, j = 1 ..r)], [seq(epsilon[j], j = 1 ..r )])[1]

$$epsilons := \left[\epsilon_1 = 0, \epsilon_2 = -iota\_theta\_y0, \epsilon_3 = -iota\_theta\_z0, \epsilon_4 = -iota\_theta\_y1, \epsilon_5 = -iota\_theta\_z1, \epsilon_6 = -\frac{iota\_theta\_z2}{K}\right] \quad (3.8)$$

**Step 3: Computing invariant vertical derivative of conformal torsion T and conformal curvature Q:**

```
> dvkappa := simplify(eval(iotadV(kappa) + eval(add(LieDerivative(g[i], kappa) · epsilon[i],
      i = 1 ..r), epsilons), cs), symbolic)
```

$$dvkappa := iota\_theta\_y2 \tag{3.9}$$

```
> dvtau := eval(iotadV(tau) + eval(add(LieDerivative(g[i], tau) · epsilon[i], i = 1 ..r),
      epsilons), cs)
```

$$dvtau := -\frac{T\ iota\_theta\_y2}{K} - \frac{K1\ iota\_theta\_z2}{K^2} + \frac{iota\_theta\_z3}{K} \tag{3.10}$$

**Computing invariant vertical derivative of ϖ:**

Here we actually compute the invariant contact form B where d_V(varpi) = B wedge varpi. (Substituting varpi = 1 amounts to hooking with invariant derivation D_sigma. Note minus sign.)

```
> B := eval(eval(eval(add(epsilon[ i] · horpart( LieDerivative(g[i], dx))  − gamma[i]
      · iotavertpart(LieDerivative(g[i], dx)), i = 1 ..r), [op(epsilons), op(gammas)]), cs),
      [varpi = 1])
```

$$B := -K\ iota\_theta\_y0 \tag{3.11}$$

**Steps 4-5: Computing the correction terms in ι(θ_i+1) = D_omega(ι(θ_i)) + corrterm_i+1.**

```
> sub := [K = K[0], K1 = K[1], T = T[0], T1 = T[1], seq(iota_theta_y || i = ICy || i[0], i = 0 ..3),
      seq(iota_theta_z || i = ICz || i[0], i = 0 ..3) ]
```

$$sub := [K = K_0, K1 = K_1, T = T_0, T1 = T_1, iota\_theta\_y0 = ICy0_0, iota\_theta\_y1 = ICy1_0, iota\_theta\_y2 = ICy2_0, iota\_theta\_y3 = ICy3_0, iota\_theta\_z0 = ICz0_0, iota\_theta\_z1 = ICz1_0, iota\_theta\_z2 = ICz2_0, iota\_theta\_z3 = ICz3_0] \tag{3.1.1}$$

```
> for j from 1 to 8 do;
  corrterm || j := eval(eval(eval(eval(horpart(add(gamma[i] LieDerivative(g[i],
      contact_forms[j]), i = 1 ..r)) + add(Hook(D_y[l], (add(gamma[i] LieDerivative(g[i],
      contact_forms[j]), i = 1 ..r)))·iota_theta_y || l, l = 0 ..10) + add(Hook(D_z[l],
      (add(gamma[i] LieDerivative(g[i], contact_forms[j]), i = 1 ..r)))·iota_theta_z || l, l = 0
      ..10), [op(epsilons), op(gammas)]), cs), [varpi = 1]), sub);
  end do:
> DGsetup([s], [K, T, seq(ICy || i, i = 0 ..3), seq(ICz || i, i = 0 ..3), f], G, 5) :
> ICforms := [seq(op([ICy || i[0], ICz || i[0]]), i = 1 ..3)] : # list of invariant contact forms
```

We now express the invariant contact forms ICy||i and ICz||i in terms of invariant derivatives of ICy0, ICz0.

```
> eq1 := ICy1[0] = ICy0[1] − corrterm1 : eq := [eq1] :
  eq2 := ICz1[0] = ICz0[1] − corrterm2 : eq := [op(eq), eq2] :
  for i from 3 to 6 do: j := i − 1 :
  eq || i := ICforms[i] = eval(TotalDiff(eval(ICforms[i − 2], eq), 1) −corrterm || i, eq) ; eq :=
      [op(eq), eq || i] :
  end do:
> eq4 # example
```

$$ICz2_0 = ICy0_0\, T_1 + T_0\, ICy0_1 + T_0\left(-T_0\, ICz0_0 + ICy0_1\right) + ICz0_2 \tag{3.1.2}$$

**Step 6: Collecting differential operators from dvT,dvK, B**

> $DGsetup([s], [K, T, seq(ICy \| i, i = 0..3), seq(ICz \| i, i = 0..3), f], G, 5):$

> $dvkappanew := expand(eval(eval(dvkappa, sub), eq));$
$dvtaunew := expand(eval(eval(dvtau, sub), eq));$
$Bnew := expand(eval(eval(B, sub), eq))$

$$dvkappanew := ICy0_0\, K_0^2 - ICy0_0\, T_0^2 - ICz0_0\, T_1 - 2\, T_0\, ICz0_1 + ICy0_2$$

$$dvtaunew := 2\, K_0\, T_0\, ICy0_0 - \frac{2\, T_0\, ICz0_0\, T_1}{K_0} - \frac{T_0^2\, ICz0_1}{K_0} + \frac{2\, T_0\, ICy0_2}{K_0} + \frac{K_1\, ICz0_0\, T_0^2}{K_0^2} - \frac{K_1\, ICy0_0\, T_1}{K_0^2} - \frac{2\, K_1\, T_0\, ICy0_1}{K_0^2} - \frac{K_1\, ICz0_2}{K_0^2} + K_0\, ICz0_1 + \frac{ICy0_0\, T_2}{K_0} + \frac{3\, T_1\, ICy0_1}{K_0} + \frac{ICz0_3}{K_0}$$

$$Bnew := -K_0\, ICy0_0 \tag{3.12}$$

**Collecting differential operators:**

> **for** $i$ **from** 0 **to** 3 **do** $Aky \| i := coeff(dvkappanew, ICy0[i])$ **end do**: **for** $i$ **from** 0 **to** 3 **do** $Akz \| i := coeff(dvkappanew, ICz0[i])$ **end do**: $simplify(dvkappanew - add(Aky \| i\ ICy0[i], i = 0..3) - add(Akz \| i\ ICz0[i], i = 0..3));$
**for** $i$ **from** 0 **to** 3 **do** $Aty \| i := coeff(dvtaunew, ICy0[i])$ **end do**: **for** $i$ **from** 0 **to** 3 **do** $Atz \| i := coeff(dvtaunew, ICz0[i])$ **end do**: $simplify(dvtaunew - add(Aty \| i\ ICy0[i], i = 0..3) - add(Atz \| i\ ICz0[i], i = 0..3));$
**for** $i$ **from** 0 **to** 3 **do** $By \| i := coeff(Bnew, ICy0[i])$ **end do**: **for** $i$ **from** 0 **to** 3 **do** $Bz \| i := coeff(Bnew, ICz0[i])$ **end do**: $simplify(Bnew - add(By \| i\ ICy0[i], i = 0..3) - add(Bz \| i\ ICz0[i], i = 0..3));$

$$0$$
$$0$$
$$0 \tag{3.13}$$

**Step 7: Computing formal adjoints**

> $Akystar := collect(expand(add(TotalDiff((-1)^j\ Aky \| j \cdot f[0], [j]), j = 0..3)), [f[3], f[2], f[1], f[0]]);$
$Akzstar := collect(expand(add(TotalDiff((-1)^j\ Akz \| j \cdot f[0], [j]), j = 0..3)), [f[3], f[2], f[1], f[0]]);$
$Atystar := collect(expand(add(TotalDiff((-1)^j\ Aty \| j \cdot f[0], [j]), j = 0..3)), [f[3], f[2], f[1], f[0]]);$
$Atzstar := collect(expand(add(TotalDiff((-1)^j\ Atz \| j \cdot f[0], [j]), j = 0..3)), [f[3], f[2], f[1], f[0]])$

$$Akystar := \left(K_0^2 - T_0^2\right) f_0 + f_2$$

$$Akzstar := 2\, T_0 f_1 + T_1 f_0$$

$$Atystar := \frac{2\, T_0 f_2}{K_0} + \left(-\frac{2\, K_1\, T_0}{K_0^2} + \frac{T_1}{K_0}\right) f_1 + 2 f_0\, K_0\, T_0$$

(3.14)

$$Atzstar := -\frac{f_3}{K_0} + \frac{2 K_1 f_2}{K_0^2} + \left(\frac{T_0^2}{K_0} - K_0 - \frac{2 K_1^2}{K_0^3} + \frac{K_2}{K_0^2}\right) f_1 - f_0 K_1 \quad \textbf{(3.14)}$$

```
> Bystar := collect(expand( add( TotalDiff( (-1)^j By||j·f[0] , [j]) ,j=0..3)),
      [f[3],f[2],f[1],f[0]]);
  Bzstar := collect(expand( add( TotalDiff( (-1)^j Bz||j·f[0] , [j]) ,j=0..3)), [f[3],
      f[2],f[1],f[0]]);
```

$$Bystar := -K_0 f_0$$

$$Bzstar := 0 \quad \textbf{(3.15)}$$

# Computing examples of SE(4)-invariant EL equations

```
> DGsetup([s], [K, T, seq(ICy||i, i=0..3), seq(ICz||i, i=0..3), f], G, 5):
```

Lagrangian = ds

```
> EL0y := eval(Bystar, [f[0]=1, seq(f[l]=0 , l=1..3)]) = 0; EL0z := eval(Bzstar,
      [f[0]=1, seq(f[l]=0 , l=1..3)]) = 0;
```

$$EL0y := -K_0 = 0$$

$$EL0z := 0 = 0 \quad \textbf{(3.16)}$$

Lagrangian = kappa ds

```
> EL1y := simplify(eval(Akystar, [f[0]=1, seq(f[l]=0 , l=1..3)]) + eval(Bystar,
      [seq(f[l]=K[l], l=0..3)])); EL1z := simplify(eval(Akzstar, [f[0]=1, seq(f[l]=0 , l
      =1..3)]) + eval(Bzstar, [seq(f[l]=K[l], l=0..3)]));
```

$$EL1y := -T_0^2$$

$$EL1z := T_1 \quad \textbf{(3.17)}$$

Lagrangian = tau ds

```
> EL2y := simplify(eval(Atystar, [f[0]=1, seq(f[l]=0 , l=1..3)]) + eval(Bystar, [seq(f[l]
      =T[l], l=0..3)])); EL2z := simplify(eval(Atzstar, [f[0]=1, seq(f[l]=0 , l=1..4)])
      + eval(Bzstar, [seq(f[l]=T[l], l=0..3)]));
```

$$EL2y := K_0 T_0$$

$$EL2z := -K_1 \quad \textbf{(3.18)}$$

Lagrangian = kappa^2 ds

```
> EL4y := simplify(eval(Akystar, [seq(f[l]=2 K[l] , l=0..3)]) + eval(Bystar, [seq(f[l]
      =TotalDiff(K[0]^2, [l]), l=0..3)])); EL4z := simplify(eval(Akzstar, [seq(f[l]
      =2 K[l] , l=0..3)]) + eval(Bzstar, [seq(f[l]=TotalDiff(K[0]^2, [l]), l=0..3)]));
```

$$EL4y := K_0^3 - 2 K_0 T_0^2 + 2 K_2$$

$$EL4z := 2 K_0 T_1 + 4 K_1 T_0 \quad \textbf{(3.19)}$$

Lagrangian = tau^2 ds

```
> EL5y := simplify(eval(Atystar, [seq(f[l]=2 T[l] , l=0..3)]) + eval(Bystar, [seq(f[l]
      =TotalDiff(T[0]^2, [l]), l=0..3)])); EL5z := simplify(eval(Atzstar, [seq(f[l]=2 T[l] ,
      l=0..3)]) + eval(Bzstar, [seq(f[l]=TotalDiff(T[0]^2, [l]), l=0..3)]));
```

$$EL5y := \frac{3\,T_0^2\,K_0^3 + 4\,T_0\,T_2\,K_0 + 2\,K_0\,T_1^2 - 4\,K_1\,T_0\,T_1}{K_0^2}$$

$$EL5z := \frac{-2\,K_0^4\,T_1 - 2\,K_1\,T_0\,K_0^3 + 2\,K_0^2\,T_0^2\,T_1 - 2\,T_3\,K_0^2 + 4\,K_1\,T_2\,K_0 + 2\,K_0\,K_2\,T_1 - 4\,K_1^2\,T_1}{K_0^3} \quad \textbf{(3.20)}$$

> solve([EL5y, EL5z], [T[2], T[3], ])[1]

$$\left[T_2 = -\frac{3\,K_0^3\,T_0^2 + 2\,K_0\,T_1^2 - 4\,K_1\,T_0\,T_1}{4\,T_0\,K_0},\ T_3 = -\frac{2\,K_0^3\,T_0\,T_1 + 5\,K_0^2\,K_1\,T_0^2 - 2\,K_0\,T_0^3\,T_1 + 2\,K_1\,T_1^2 - 2\,K_2\,T_0\,T_1}{2\,T_0\,K_0}\right] \quad \textbf{(3.21)}$$

## Computing W:

> $DGsetup([x], [y, z], E, 12)$ :

> omega := $evalDG\left(\frac{1}{Ts(x)}\ dx\right)$ :# *omega = ds arc length parameter*

$vt1 := evalDG\left(\frac{1}{Ts(x)^2}\ (\ diff(\text{kappa}, y[2])\cdot(dy[0] - y[1]\,dx) + \ diff(\text{kappa}, z[2])\cdot(dz[0] - z[1]\,dx)\ )\right)$ : # *invariant contact form of order 0 constructed from symbol of kappa*

$vt2 := evalDG\left(\frac{\text{kappa}}{Ts(x)^3}\ (\ diff(\text{tau}, y[3])\cdot(dy[0] - y[1]\,dx) + \ diff(\text{tau}, z[3])\cdot(dz[0] - z[1]\,dx)\ )\right)$ : # *invariant contact form of order 0 constructed from symbol of tau*

> $simplify(eval([vt1, vt2], cs), symbolic)$
# *vt1,vt2 are invariantizations of theta_y0 and theta_z0 respectively*

$$\left[0\,dx + dy_0 + 0\,dz_0,\ 0\,dx + 0\,dy_0 + dz_0\right] \quad \textbf{(3.2.1)}$$

> solve(DGinfo(evalDG(vt1 &w omega − W1y·(dy[0]−y[1]·dx) &w dx − W1z ·(dz[0]−z[1]·dx) &w dx), "CoefficientSet") **union** DGinfo(evalDG(vt2 &w omega − W2y·(dy[0]−y[1]·dx) &w dx − W2z·(dz[0]−z[1]·dx) &w dx), "CoefficientSet"), [W1y, W1z, W2y, W2z])[1] : Wlocal := simplify(eval(Matrix([[W1y, W1z], [W2y, W2z]]), %), symbolic);
Determinant(Wlocal)

$Wlocal :=$

$$\begin{bmatrix} \frac{-y_1\,z_1\,z_2 + y_2\,z_1^2 + y_2}{\sqrt{(z_1^2+1)\,y_2^2 - 2\,y_1\,y_2\,z_1\,z_2 + z_2^2\,(y_1^2+1)}} & \frac{y_1^2\,z_2 - y_1\,y_2\,z_1 + z_2}{\sqrt{(z_1^2+1)\,y_2^2 - 2\,y_1\,y_2\,z_1\,z_2 + z}} \cdots \\ -\frac{z_2\,\sqrt{y_1^2+z_1^2+1}}{\sqrt{(z_1^2+1)\,y_2^2 - 2\,y_1\,y_2\,z_1\,z_2 + z_2^2\,(y_1^2+1)}} & \frac{y_2\,\sqrt{y_1^2+z_1^2+1}}{\sqrt{(z_1^2+1)\,y_2^2 - 2\,y_1\,y_2\,z_1\,z_2 + z}} \cdots \end{bmatrix}$$

$$\sqrt{y_1^2 + z_1^2 + 1} \quad \textbf{(3.2.2)}$$

**Global invariant coframe:**

```
> omega2 := evalDG( 1/(kappa kappa1 Ts(x)) · dx ) :
  varthetay := evalDG( 1/(1 + y[1]^2 + z[1]^2)^2 ·( ((1 + z[1]^2) y[2] − y[1] z[1] z[2] )
    · (dy[0] − y[1] dx)   +  ((1 + y[1]^2) z[2] − y[1] z[1] y[2] ) ·(dz[0]
    − z[1] dx)       )) :
  varthetaz := evalDG( kappa1/(sqrt( (y[1] z[2] − y[2] z[1])^2 + y[2]^2 + z[2]^2 )) · ( −z[2]
    ·(dy[0] − y[1] dx) +  y[2]·(dz[0] − z[1] dx) ) ) :
```

```
> simplify(eval([varthetay, varthetaz], cs), symbolic)
```

$$\left[0\,dx + K\,dy_0 + 0\,dz_0,\ 0\,dx + 0\,dy_0 + K1\,dz_0\right] \qquad (3.2.3)$$

Computing Wglobal:

```
> solve(DGinfo(evalDG(varthetay &w omega2 − W11·(dy[0]−y[1]·dx) &w dx − W12 ·(dz[0]
    −z[1]·dx) &w dx), "CoefficientSet") union DGinfo(evalDG(varthetaz &w omega2
    − W21·(dy[0]−y[1]·dx) &w dx − W22·(dz[0]−z[1]·dx) &w dx), "CoefficientSet"),
    [W11, W12, W21, W22])[1] : Wglobal := simplify(eval(Matrix([[W11, W12], [W21,
    W22]]), %), symbolic)
```

Wglobal := (3.2.4)

$$\left[\begin{array}{l} -\frac{\cdots}{y_2 y_3 z_1^4 + \left(\left(-y_2 z_3 - y_3 z_2\right) y_1 - 3\,y_2^2 z_2\right) z_1^3 + \left(\left(y_2 y_3 + z_2 z_3\right) y_1^2 + \left(-3\,y_2^3 + \cdots\right.\right.} \\ \cdots \end{array}\right]$$

```
> simplify(Wglobal − MatrixMatrixMultiply(DiagonalMatrix([κ1^-1,  κ^-1]), Wlocal) ,
    symbolic)
```

$$\begin{bmatrix} 0 & 0 \\ 0 & 0 \end{bmatrix} \qquad (3.2.5)$$

**Conclusion:** Wglobal = diag(kappa1^-1, kappa^-1).Wlocal

# Conformal 3D

```
> restart : with(DifferentialGeometry) : with(LieAlgebras) : with(Tensor) : with(GroupActions) :
    with(Tools) : Preferences("ShowFramePrompt",'false') : interface(warnlevel = 0) :
    with(LinearAlgebra) : with(PDETools) : with(JetCalculus) : with(ArrayTools) :
    Preferences("JetNotation", "JetNotation2") :
```

```
> DGsetup([x], [y, z], E, 12) : totalD := evalDG(D_x + add(y[i + 1] D_y[i], i = 0 ..10 )
    + add(z[i + 1] D_z[i], i = 0 ..10 )) : contact_forms := [seq(op([dy[i] − y[i + 1] dx,
    dz[i] − z[i + 1] dx]), i = 0 ..8)] :
```

**Lie algebra of conformal group:**

```
> conf := evalDG([D_x, D_y[0], D_z[0], x D_y[0] - y[0] D_x, x D_z[0] - z[0] D_x,
    y[0] D_z[0] - z[0] D_y[0], x D_x + y[0] D_y[0] + z[0] D_z[0], 1/2·(x^2 + y[0]^2
    + z[0]^2) D_x - x·(x D_x + y[0] D_y[0] + z[0] D_z[0]), 1/2·(x^2 + y[0]^2
    + z[0]^2) D_y[0] - y[0]·(x D_x + y[0] D_y[0] + z[0] D_z[0]), 1/2·(x^2 + y[0]^2
    + z[0]^2) D_z[0] - z[0]·(x D_x + y[0] D_y[0] + z[0] D_z[0])]) : g :=
    map(Prolong, conf, 10) : r := nops(conf) :
```

**Local invariants:**

Euclidean invariants:

```
> R1 := y[1]^2 + z[1]^2 + 1 : R2 := (y[1]^2 + 1) z[2]^2 - 2 y[1] z[1] y[2] z[2] + (z[1]^2
    + 1) y[2]^2 : R3a := z[2] y[3]-y[2] z[3] : Ts := f -> 1/sqrt(R1) TotalDiff(f, x) :
  kappa := simplify(sqrt(R2/R1^3), symbolic) : κ0 := κ :for i to 4 do κ||i := Ts(κ||(i - 1)):od:

  tau := simplify(-R3a/R2) : τ0 := τ : for i to 4 do τ||i := Ts(τ||(i - 1)):od:
  nu := simplify(sqrt(κ1^2 + κ^2 τ^2), symbolic) : # relative conformal invariant
```

Conformal torsion T and conformal curvature Q are scalar diff invariants of order 4 and order 5, respectively.

```
> Domega := f -> 1/sqrt(nu) Ts(f) : # conformal arclength, invariant derivation
```

```
> T := simplify((2 κ1^2 τ + κ^2 τ^3 + κ kappa1 τ1 - kappa kappa2 τ)/(ν)^(5/2), symbolic) : T0 := T :
    for i to 2 do T||i := Domega(T||(i - 1)):od:
  Q := simplify((4 (Ts(Ts(nu)) - κ^2 ν) ν - 5 Ts(ν)^2)/(8 ν^3), symbolic) : Q0 := Q :for i to 2
    do Q||i := Domega(Q||(i - 1)):od:
```

```
> seq(simplify(LieDerivative(g[i], [T, Q])), i = 1..10)
      [0, 0], [0, 0], [0, 0], [0, 0], [0, 0], [0, 0], [0, 0], [0, 0], [0, 0], [0, 0]      (4.1)
```

## Computing cross-section

> $V := evalDG(add(a\|i\, g[i] \quad , i = 1..10)):$

> $eval(LieDerivative(V, [x, y[0], z[0]]), [\ ])$
  # We can set first three coordinates equal to zero by using translations, i.e., a1 = a2 = a3 = 0

$$\Big[-a10\, x\, z_0 - a9\, x\, y_0 - \frac{1}{2}\, a8\, x^2 + \frac{1}{2}\, a8\, y_0^2 + \frac{1}{2}\, a8\, z_0^2 - a4\, y_0 - a5\, z_0 + a7\, x + a1, \quad -a10\, y_0\, z_0 + \frac{1}{2}\, a9\, x^2 - \frac{1}{2}\, a9\, y_0^2 + \frac{1}{2}\, a9\, z_0^2 - a8\, x\, y_0 + a4\, x - a6\, z_0 + a7\, y_0 + a2, \quad \frac{1}{2}\, a10\, x^2 + \frac{1}{2}\, a10\, y_0^2 - \frac{1}{2}\, a10\, z_0^2 - a8\, x\, z_0 - a9\, y_0\, z_0 + a5\, x + a6\, y_0 + a7\, z_0 + a3\Big] \quad \textbf{(4.1.1)}$$

> $eval(LieDerivative(V, [x, y[0], z[0]]), [x = 0, y[0] = 0, z[0] = 0, a1 = 0, a2 = 0, a3 = 0])$

$$[0, 0, 0] \quad \textbf{(4.1.2)}$$

> $eval(LieDerivative(V, [y[1], z[1]]), [x = 0, y[0] = 0, z[0] = 0, a1 = 0, a2 = 0, a3 = 0])$

$$\left[a4\, y_1^2 + a5\, y_1\, z_1 - a6\, z_1 + a4,\ a4\, y_1\, z_1 + a5\, z_1^2 + a6\, y_1 + a5\right] \quad \textbf{(4.1.3)}$$

> $eval(LieDerivative(V, [y[1], z[1]]), [x = 0, y[0] = 0, z[0] = 0, y[1] = 0, z[1] = 0, a1 = 0, a2 = 0, a3 = 0, a4 = 0, a5 = 0])$

$$[0, 0] \quad \textbf{(4.1.4)}$$

> $eval(LieDerivative(V, [y[2], z[2]]), [x = 0, y[0] = 0, z[0] = 0, y[1] = 0, z[1] = 0, a1 = 0, a2 = 0, a3 = 0, a4 = 0, a5 = 0])$

$$\left[-a6\, z_2 - a7\, y_2 + a9,\ a6\, y_2 - a7\, z_2 + a10\right] \quad \textbf{(4.1.5)}$$

> $eval(LieDerivative(V, [y[2], z[2]]), [x = 0, y[0] = 0, z[0] = 0, y[1] = 0, z[1] = 0, y[2] = 0, z[2] = 0, a1 = 0, a2 = 0, a3 = 0, a4 = 0, a5 = 0, a9 = 0, a10 = 0])$

$$[0, 0] \quad \textbf{(4.1.6)}$$

> $eval(LieDerivative(V, [y[3], z[3]]), [x = 0, y[0] = 0, z[0] = 0, y[1] = 0, z[1] = 0, y[2] = 0, z[2] = 0, a1 = 0, a2 = 0, a3 = 0, a4 = 0, a5 = 0, a9 = 0, a10 = 0])$
  # consist of rotation and dilatation, so we can set y3 = 1, z_3 = 0

$$\left[-a6\, z_3 - 2\, a7\, y_3,\ a6\, y_3 - 2\, a7\, z_3\right] \quad \textbf{(4.1.7)}$$

> $eval(LieDerivative(V, [y[3], z[3]]), [x = 0, y[0] = 0, z[0] = 0, y[1] = 0, z[1] = 0, y[2] = 0, z[2] = 0, y[3] = 1, z[3] = 0, a1 = 0, a2 = 0, a3 = 0, a4 = 0, a5 = 0, a6 = 0, a7 = 0, a9 = 0, a10 = 0])$

$$[0, 0] \quad \textbf{(4.1.8)}$$

> $eval(LieDerivative(V, [y[4], z[4]]), [x = 0, y[0] = 0, z[0] = 0, y[1] = 0, z[1] = 0, y[2] = 0, z[2] = 0, y[3] = 1, z[3] = 0, a1 = 0, a2 = 0, a3 = 0, a4 = 0, a5 = 0, a6 = 0, a7 = 0, a9 = 0, a10 = 0])$

$$[2\, a8, 0] \quad \textbf{(4.1.9)}$$

> $eval(LieDerivative(V, [y[4], z[4]]), [x = 0, y[0] = 0, z[0] = 0, y[1] = 0, z[1] = 0, y[2] = 0, z[2] = 0, y[3] = 1, z[3] = 0, y[4] = 0, a1 = 0, a2 = 0, a3 = 0, a4 = 0, a5 = 0, a6 = 0, a7 = 0, a8 = 0, a9 = 0, a10 = 0])$

$$[0, 0] \quad \textbf{(4.1.10)}$$

Defining cross-section:

> $cs0 := [x = 0, y[0] = 0, z[0] = 0, y[1] = 0, z[1] = 0, y[2] = 0, z[2] = 0, y[3] = 1, z[3] = 0, y[4] = 0];$ # cross-section

$$cs0 := \left[x = 0, y_0 = 0, z_0 = 0, y_1 = 0, z_1 = 0, y_2 = 0, z_2 = 0, y_3 = 1, z_3 = 0, y_4 = 0\right] \quad \textbf{(4.2)}$$

**Relating invariantization to conformal invariants:**

> $eval([t=T, q=Q, t1=T1], cs0);\ invariantizations := solve(\%, [z[4], y[5], z[5]])[1]$

$$\left[t=z_4,\ q=\frac{z_4^2}{2}+\frac{y_5}{2},\ t1=z_5\right]$$

$$invariantizations := \left[z_4=t,\ y_5=-t^2+2\,q,\ z_5=t1\right] \qquad (4.3)$$

> $cs := [\ op(cs0), op(invariantizations), d\_x=\mathrm{varpi}\ ];$
> # *updating cross-section to include T, Q, T1 and varpi as invariantizations*

$$cs := \left[x=0,\ y_0=0,\ z_0=0,\ y_1=0,\ z_1=0,\ y_2=0,\ z_2=0,\ y_3=1,\ z_3=0,\ y_4=0,\ z_4=t,\ y_5=-t^2+2\,q,\ z_5=t1,\ d\_x=\varpi\right] \qquad (4.4)$$

**Step 1: Defining horizontal and vertical derivative, horizontal and vertical component of a one-form on J^infinity, as well as iota composed with dV and vertpart.**

> $horpart := \mathrm{eta} \to Hook(totalD, \mathrm{eta})\cdot d\_x :$
> # *horizontal part of a one-form (NB: d_x is a symbol!)*
> $vertpart := \mathrm{eta} \to add(Hook(D\_y[i], \mathrm{eta})\cdot cat(theta\_y, i) + Hook(D\_z[i], \mathrm{eta})\cdot cat(theta\_z, i), i=0..12) :$ # *vertical part of a one-form*
> $dH := f \to Hook(totalD, ExteriorDerivative(f)\ )\cdot d\_x :$ # *horizontal derivative of a function*
> $dV := f \to\ vertpart(\,VerticalExteriorDerivative(f)\ ) :$ # *vertical derivative of a function*
> $iotavertpart := \mathrm{eta} \to add(eval(Hook(D\_y[i], \mathrm{eta}), cs)\cdot cat(iota\_theta\_y, i) + eval(Hook(D\_z[i], \mathrm{eta}), cs)\cdot cat(iota\_theta\_z, i), i=0..12) :$
> # *iota composed with vertical part of one-form*
> $iotadV := f \to\ add(eval(Hook(D\_y[i], ExteriorDerivative(f), cs)\cdot cat(iota\_theta\_y, i) + Hook(D\_z[i], ExteriorDerivative(f), cs)\cdot cat(iota\_theta\_z, i)\ \ ), i=0..10) :$
> # *iota composed with dV*

**Step 2: Computing gamma and epsilon terms**

> $csvars := map(lhs, cs0) :$ # *list of variables that are constant on cross-section*

> **for** $j$ **from** 1 **to** $r$ **do**;
> $gam \| j := eval(dH(csvars[j]) + add(LieDerivative(g[i], csvars[j])\cdot \mathrm{gamma}[i], i=1..r), cs) :$ #
> **end do**:
> $gammas := solve([seq(gam \| j=0, j=1..r)], [seq(\mathrm{gamma}[j], j=1..r)])[1]$

$$gammas := \left[\gamma_1=-\varpi,\ \gamma_2=0,\ \gamma_3=0,\ \gamma_4=0,\ \gamma_5=0,\ \gamma_6=-t\,\varpi,\ \gamma_7=0,\ \gamma_8=-q\,\varpi,\ \gamma_9=-\varpi,\ \gamma_{10}=0\right] \qquad (4.5)$$

> **for** $j$ **from** 1 **to** $r$ **do**;
> $eps \| j := iotadV(csvars[j]) + eval(add(LieDerivative(g[i], csvars[j]\cdot \mathrm{epsilon}[i]), i=1..r), cs) :$
> **end do**:
> $epsilons := solve([seq(eps \| j=0, j=1..r)],\ [seq(\mathrm{epsilon}[j], j=1..r\ )])[1]$

$$epsilons := \left[\epsilon_1=0,\ \epsilon_2=-iota\_theta\_y0,\ \epsilon_3=-iota\_theta\_z0,\ \epsilon_4=-iota\_theta\_y1,\ \epsilon_5=-iota\_theta\_z1,\ \epsilon_6=-iota\_theta\_z3,\ \epsilon_7=\frac{iota\_theta\_y3}{2},\ \epsilon_8=-\frac{t\,iota\_theta\_z3}{2}\right. \qquad (4.6)$$

$$-\frac{iota\_theta\_y4}{2}, \epsilon_9 = -iota\_theta\_y2, \epsilon_{10} = -iota\_theta\_z2\Big]$$

**Step 3: Computing invariant vertical derivative of conformal torsion T and conformal curvature Q:**

> $dvT := eval(iotadV(T) + eval(add(LieDerivative(g[i],\ T)\cdot \text{epsilon}[i], i=1..r), epsilons), cs)$

$$dvT := -\frac{3\ t\ iota\_theta\_y3}{2} + iota\_theta\_z4 \qquad \textbf{(4.7)}$$

> $dvQ := eval(iotadV(Q) + eval(add(LieDerivative(g[i],\ Q)\cdot \text{epsilon}[i], i=1..r), epsilons), cs)$

$$dvQ := -5\ iota\_theta\_y1 + \frac{(-4\ t^2 - 16\ q)\ iota\_theta\_y3}{8} + \frac{t1\ iota\_theta\_z3}{2} + t\ iota\_theta\_z4 + \frac{iota\_theta\_y5}{2} \qquad \textbf{(4.8)}$$

**Computing invariant vertical derivative of ϖ:**

Here we actually compute the invariant contact form B where d_V(varpi) = B wedge varpi. (Substituting varpi = 1 amounts to hooking with invariant derivation D_sigma. Note minus sign.)

> $B := eval(eval(eval(add(\text{epsilon}[\ i]\cdot horpart(\ LieDerivative(g[i],\ dx)) - \text{gamma}[i] \cdot iotavertpart(LieDerivative(g[i],\ dx)), i\ = 1..r), [op(epsilons), op(gammas)]), cs), [\text{varpi} = 1])$

$$B := \frac{iota\_theta\_y3}{2} \qquad \textbf{(4.9)}$$

**Steps 4-5: Computing the correction terms in ι(θ_i+1) = D_omega(ι(θ_i)) + corrterm_i+1.**

> $sub := [q = q[0], q1 = q[1], t = t[0], t1 = t[1], seq(iota\_theta\_y \| i = ICy \| i[0], i = 0..5), seq(iota\_theta\_z \| i = ICz \| i[0], i = 0..5)\ ]$

$$sub := \big[q = q_0, q1 = q_1, t = t_0, t1 = t_1, iota\_theta\_y0 = ICy0_0, iota\_theta\_y1 = ICy1_0, iota\_theta\_y2 = ICy2_0, iota\_theta\_y3 = ICy3_0, iota\_theta\_y4 = ICy4_0, iota\_theta\_y5 = ICy5_0, iota\_theta\_z0 = ICz0_0, iota\_theta\_z1 = ICz1_0, iota\_theta\_z2 = ICz2_0, iota\_theta\_z3 = ICz3_0, iota\_theta\_z4 = ICz4_0, iota\_theta\_z5 = ICz5_0\big] \qquad \textbf{(4.2.1)}$$

```
> for j from 1 to 10 do;
  corrterm || j := eval(eval(eval(eval(horpart(add(gamma[i] LieDerivative(g[i],
      contact_forms[j]), i = 1 ..r)) + add(Hook(D_y[l], (add(gamma[i] LieDerivative(g[i],
      contact_forms[j]), i = 1 ..r)))·iota_theta_y || l , l = 0 ..10) + add(Hook(D_z[l],
      (add(gamma[i] LieDerivative(g[i], contact_forms[j]), i = 1 ..r)))·iota_theta_z || l , l = 0
      ..10), [op(epsilons), op(gammas)]), cs), [varpi = 1]), sub);
  end do:
> DGsetup([s], [q, t, seq(ICy || i, i = 0 ..5), seq(ICz || i, i = 0 ..5), f], G, 5) :
```

We express invariant contact forms IC||i[0] in terms of a IC0[0], ICO[1], etc (i.e., as a differential operator acting on IC0[0]'s)

```
> eq1 := IC1[0] = IC0[1] − corrterm1 : eq := [eq1] :
   for i from 2 to 6 do: j := i − 1 :
  eq || i := IC || i[0] = eval(TotalDiff(eval(IC || j[0], eq), 1) −corrterm || i, eq) ; eq := [op(eq),
```

$eq\|i]$ :
**end do**:

> $ICforms := [seq(op([ICy\|i[0], ICz\|i[0]]), i = 1..5)]$ :

> $eq1 := ICy1[0] = ICy0[1] - corrterm1 : eq := [eq1]$ :
$eq2 := ICz1[0] = ICz0[1] - corrterm2 : eq := [op(eq), eq2]$ :
**for** $i$ **from** 3 **to** 10 **do**: $j := i - 1$ :
$eq\|i := ICforms[i] = eval(TotalDiff(eval(ICforms[i-2], eq), 1) - corrterm\|i, eq)$ ; $eq :=$
$[op(eq), eq\|i]$ :
**end do**:

> $eq4$ # example

$$ICz2_0 = ICy0_0\, t_1 + t_0\, ICy0_1 + \left(-t_0\, ICz0_0 + ICy0_1\right) t_0 - ICz0_0\, q_0 + ICz0_2 \qquad \textbf{(4.2.2)}$$

**Step 6: Collecting differential operators from dvT,dvK, B**

> $DGsetup([s], [q, t, seq(ICy\|i, i = 0..5), seq(ICz\|i, i = 0..5), f], G, 5)$ :

> $dvTnew := expand(eval(eval(dvT, sub), eq))$;
$dvQnew := expand(eval(eval(dvQ, sub), eq))$;
$Bnew := expand(eval(eval(B, sub), eq))$

$$dvTnew := -ICz0_0 + 6\, t_1\, ICy0_2 - ICz0_0\, q_2 + ICy0_0\, t_3 - \frac{15}{2}\, ICz0_1\, t_0\, t_1 + ICz0_4 - \frac{3}{2}\, ICy0_0\, t_0^2\, t_1 - \frac{1}{2}\, ICz0_0\, t_0^4 + \frac{1}{2}\, ICy0_1\, t_0^3 - \frac{3}{2}\, ICz0_2\, t_0^2 + 4\, ICy0_1\, t_2 - 3\, ICz0_1\, q_1 - 2\, ICz0_2\, q_0 - 3\, ICz0_0\, t_1^2 - \frac{5}{2}\, ICz0_0\, t_0\, t_2 + \frac{5}{2}\, t_0\, ICy0_3 - ICy0_1\, q_0\, t_0 - \frac{3}{2}\, ICy0_0\, q_1\, t_0 - ICz0_0\, q_0\, t_0^2 - 2\, ICy0_0\, q_0\, t_1$$

$$dvQnew := 2\, ICy0_1 - \frac{1}{2}\, ICy0_0\, q_3 + \frac{1}{2}\, ICy0_5 - t_0\, ICz0_0 + 3\, ICy0_0\, q_0\, t_0\, t_1 + ICy0_0\, q_0\, q_1 + 2\, ICz0_0\, q_0\, t_2 + 3\, ICz0_0\, t_0\, t_1^2 + 2\, ICz0_1\, q_1\, t_0 - \frac{15}{2}\, ICy0_2\, t_0\, t_1 + \frac{3}{2}\, ICz0_0\, t_0^2\, t_2 + 4\, ICz0_2\, q_0\, t_0 - \frac{3}{2}\, ICy0_0\, t_0\, t_3 - 6\, ICy0_1\, t_0\, t_2 + ICz0_0\, q_2\, t_0 + 3\, ICy0_1\, q_0\, t_0^2 - ICz0_0\, q_0\, t_0^3 - \frac{9}{2}\, ICy0_0\, t_1\, t_2 - 2\, ICz0_0\, q_0^2\, t_0 + 5\, ICz0_1\, q_0\, t_1 + 2\, ICz0_0\, q_1\, t_1 + 3\, ICz0_1\, t_0^2\, t_1 - \frac{9}{2}\, t_1\, ICz0_3 - \frac{3}{2}\, t_0\, ICz0_4 - \frac{1}{2}\, ICz0_0\, t_4 + \frac{1}{2}\, ICz0_2\, t_0^3 + 2\, ICy0_1\, q_0^2 - \frac{3}{2}\, ICy0_3\, t_0^2 - 2\, ICy0_3\, q_0 - 6\, ICy0_1\, t_1^2 - 2\, ICy0_1\, q_2 - \frac{5}{2}\, ICy0_2\, q_1 - \frac{5}{2}\, ICz0_1\, t_3 - 5\, ICz0_2\, t_2$$

$$Bnew := -\frac{3}{2}\, ICy0_1\, t_0^2 - ICy0_1\, q_0 + \frac{1}{2}\, ICy0_3 - \frac{3}{2}\, t_1\, ICz0_1 - \frac{3}{2}\, t_0\, ICz0_2 - \frac{1}{2}\, ICy0_0\, q_1 - \frac{3}{2}\, ICy0_0\, t_0\, t_1 - \frac{1}{2}\, ICz0_0\, t_2 + ICz0_0\, q_0\, t_0 + \frac{1}{2}\, ICz0_0\, t_0^3 \qquad \textbf{(4.10)}$$

**Collecting differential operators:**

> **for** $i$ **from** 0 **to** 5 **do** $ATy\|i := coeff(dvTnew, ICy0[i])$ **end do**: **for** $i$ **from** 0 **to** 5 **do** $ATz$
$\|i := coeff(dvTnew, ICz0[i])$ **end do**: $simplify(dvTnew - add(ATy\|i\ ICy0[i], i = 0..5))$

```
    - add(ATz || i ICz0[i], i = 0 ..5) );
  for i from 0 to 5 do AQy || i := coeff(dvQnew, ICy0[i]) end do: for i from 0 to 5 do AQz
    || i := coeff(dvQnew, ICz0[i]) end do: simplify(dvQnew - add(AQy || i ICy0[i], i = 0 ..5)
    - add(AQz || i ICz0[i], i = 0 ..5) );
  for i from 0 to 5 do By || i := coeff(Bnew, ICy0[i]) end do: for i from 0 to 5 do Bz || i :=
    coeff(Bnew, ICz0[i]) end do: simplify(Bnew - add(By || i ICy0[i], i = 0 ..5) - add(Bz
    || i ICz0[i], i = 0 ..5) );;
```

$$0$$

$$0$$

$$0 \tag{4.11}$$

**Step 7: Computing formal adjoints**

```
> ATystar := collect(expand( add( TotalDiff( (-1)^j ATy||j ·f[0] , [j]) ,j = 0 ..5)),
      [f[5],f[4],f[3],f[2],f[1],f[0]]);
  ATzstar := collect(expand( add( TotalDiff( (-1)^j ATz||j ·f[0] , [j]) ,j = 0 ..5)),
      [f[5],f[4],f[3],f[2],f[1],f[0]]) ;
  AQystar := collect(expand( add( TotalDiff( (-1)^j AQy||j ·f[0] , [j]) ,j = 0 ..5)),
      [f[5],f[4],f[3],f[2],f[1],f[0]]) ;
  AQzstar := collect(expand( add( TotalDiff( (-1)^j AQz||j ·f[0] , [j]) ,j = 0 ..5)),
      [f[5],f[4],f[3],f[2],f[1],f[0]])
```

$$ATystar := -\frac{5\, t_0 f_3}{2} - \frac{3\, t_1 f_2}{2} + \left(-\frac{1}{2}\, t_0^3 + \frac{1}{2}\, t_2 + t_0\, q_0\right) f_1 + \left(\frac{1}{2}\, t_3 - 3\, t_0^2\, t_1 - \frac{1}{2}\, t_0\, q_1 - q_0\, t_1\right) f_0$$

$$ATzstar := f_4 + \left(-\frac{3\, t_0^2}{2} - 2\, q_0\right) f_2 + \left(\frac{3\, t_0\, t_1}{2} - q_1\right) f_1 + \left(-1 - \frac{1}{2}\, t_0^4 + \frac{3}{2}\, t_1^2 + 2\, t_0\, t_2 - q_0\, t_0^2\right) f_0$$

$$AQystar := -\frac{f_5}{2} + \left(\frac{3\, t_0^2}{2} + 2\, q_0\right) f_3 + \left(\frac{7\, q_1}{2} + \frac{3\, t_0\, t_1}{2}\right) f_2 + \left(-3\, q_0\, t_0^2 - 2\, q_0^2 + 3\, q_2 - 2\right) f_1 + \left(-3\, q_0\, t_0\, t_1 - 3\, q_1\, t_0^2 - 3\, q_0\, q_1 + q_3\right) f_0$$

$$AQzstar := -\frac{3\, t_0 f_4}{2} - \frac{3\, t_1 f_3}{2} + \left(-\frac{1}{2}\, t_2 + \frac{1}{2}\, t_0^3 + 4\, t_0\, q_0\right) f_2 + \left(3\, q_0\, t_1 + 6\, t_0\, q_1\right) f_1 + \left(-q_0\, t_0^3 - 2\, q_0^2\, t_0 + q_0\, t_2 + 3\, q_1\, t_1 + 3\, q_2\, t_0 - t_0\right) f_0 \tag{4.12}$$

```
> Bystar := collect(expand( add( TotalDiff( (-1)^j By||j ·f[0] , [j]) ,j = 0 ..5)), [f[5],
      f[4],f[3],f[2],f[1],f[0]]);
  Bzstar := collect(expand( add( TotalDiff( (-1)^j Bz||j ·f[0] , [j]) ,j = 0 ..5)), [f[5],
      f[4],f[3],f[2],f[1],f[0]]);
```

$$Bystar := -\frac{f_3}{2} + \left(\frac{3\, t_0^2}{2} + q_0\right) f_1 + \left(\frac{q_1}{2} + \frac{3\, t_0\, t_1}{2}\right) f_0$$

$$Bzstar := \left(-\frac{1}{2}\, t_2 + t_0\, q_0 + \frac{1}{2}\, t_0^3\right) f_0 - \frac{3\, t_1\, f_1}{2} - \frac{3\, t_0\, f_2}{2} \tag{4.13}$$

# Computing examples of conformally invariant EL equations:

**We substitute Eulerian into Astar and Hamiltonian into Bstar.**

Lagrangian = omega

> *EL0y* := *eval*(*Bystar*, [*f*[0] = 1, *seq*(*f*[*l*] = 0 , *l* = 1 ..5)]) = 0; *EL0z* := *eval*(*Bzstar*, [*f*[0] = 1, *seq*(*f*[*l*] = 0 , *l* = 1 ..5)]) = 0

$$EL0y := \frac{q_1}{2} + \frac{3\, t_0\, t_1}{2} = 0$$

$$EL0z := -\frac{1}{2}\, t_2 + t_0\, q_0 + \frac{1}{2}\, t_0^3 = 0 \tag{4.14}$$

> *solve*([*EL0y*, *EL0z*], [*q*[1], *t*[2]])[1]

$$\left[q_1 = -3\, t_0\, t_1,\, t_2 = t_0^3 + 2\, t_0\, q_0\right] \tag{4.15}$$

Lagrangian = T omega

> *EL1y* := *simplify*(*eval*(*ATystar*, [*f*[0] = 1, *seq*(*f*[*l*] = 0 , *l* = 1 ..5)]) + *eval*(*Bystar*, [*seq*(*f*[*l*] = *t*[*l*], *l* = 0 ..5)])); *EL1z* := *simplify*(*eval*(*ATzstar*, [*f*[0] = 1, *seq*(*f*[*l*] = 0 , *l* = 1 ..5)]) + *eval*(*Bzstar*, [*seq*(*f*[*l*] = *t*[*l*], *l* = 0 ..5)]))

$$EL1y := 0$$

$$EL1z := -1 \tag{4.16}$$

**No regular extremals! This is expected because we know that conformal torsion is Lagrangian for conformal geodesics and conformal geodesics are given by a third-order equation.**

Lagrangian = Q omega

> *EL2y* := *simplify*(*eval*(*AQystar*, [*f*[0] = 1, *seq*(*f*[*l*] = 0 , *l* = 1 ..5)]) + *eval*(*Bystar*, [*seq*(*f*[*l*] = *q*[*l*], *l* = 0 ..5)])); *EL2z* := *simplify*(*eval*(*AQzstar*, [*f*[0] = 1, *seq*(*f*[*l*] = 0 , *l* = 1 ..5)]) + *eval*(*Bzstar*, [*seq*(*f*[*l*] = *q*[*l*], *l* = 0 ..5)]))

$$EL2y := \frac{\left(-3\, t_0^2 - 3\, q_0\right) q_1}{2} - \frac{3\, q_0\, t_0\, t_1}{2} + \frac{q_3}{2}$$

$$EL2z := -\frac{q_0\, t_0^3}{2} + \frac{\left(-2\, q_0^2 + 3\, q_2 - 2\right) t_0}{2} + \frac{q_0\, t_2}{2} + \frac{3\, q_1\, t_1}{2} \tag{4.17}$$

> *solve*([*EL2y*, *EL2z*], [*q*[3], *q*[2]])[1]

$$\left[q_3 = 3\, q_0\, t_0\, t_1 + 3\, q_1\, t_0^2 + 3\, q_0\, q_1,\, q_2 = -\frac{-q_0\, t_0^3 - 2\, q_0^2\, t_0 + q_0\, t_2 + 3\, q_1\, t_1 - 2\, t_0}{3\, t_0}\right] \tag{4.18}$$

Lagrangian = T^2 omega

> *EL3y* := *simplify*(*eval*(*ATystar*, [*seq*(*f*[*l*] = 2 *t*[*l*] , *l* = 0 ..5)]) + *eval*(*Bystar*, [*seq*(*f*[*l*] = *TotalDiff*(*t*[0]^2, [*l*]), *l* = 0 ..5)])); *EL3z* := *simplify*(*eval*(*ATzstar*, [*seq*(*f*[*l*] = 2 *t*[*l*] , *l* = 0 ..5)]) + *eval*(*Bzstar*, [*seq*(*f*[*l*] = *TotalDiff*(*t*[0]^2, [*l*]), *l* = 0 ..5)]))

$$EL3y := -5\, t_0\, t_3 - 5\, t_1\, t_2 - \frac{5}{2}\, t_1\, t_0^3 + 2\, q_0\, t_0\, t_1 - \frac{1}{2}\, q_1\, t_0^2$$

**(4.19)**

$$EL3z := 2\,t_4 - \frac{5}{2}\,t_0^2\,t_2 - 4\,q_0\,t_2 - 2\,q_1\,t_1 - 2\,t_0 - \frac{1}{2}\,t_0^5 - q_0\,t_0^3 \quad \textbf{(4.19)}$$

> $solve([EL3y, EL3z], [t[4], t[3]])[1]$

$$\left[t_4 = \frac{1}{4}\,t_0^5 + \frac{1}{2}\,q_0\,t_0^3 + \frac{5}{4}\,t_0^2\,t_2 + 2\,q_0\,t_2 + q_1\,t_1 + t_0,\ t_3 = -\frac{5\,t_1\,t_0^3 - 4\,q_0\,t_0\,t_1 + q_1\,t_0^2 + 10\,t_1\,t_2}{10\,t_0}\right] \quad \textbf{(4.20)}$$

Lagrangian = Q^2 omega

> $EL4y := simplify(eval(AQystar, [seq(f[l]=2\,q[l], l=0..5)]) + eval(Bystar, [seq(f[l] = TotalDiff(q[0]^2, [l]), l=0..5)])); EL4z := simplify(eval(AQzstar, [seq(f[l]=2\,q[l], l=0..5)]) + eval(Bzstar, [seq(f[l] = TotalDiff(q[0]^2, [l]), l=0..5)]))$

$$EL4y := \frac{\left(-18\,q_0\,t_0^2 - 15\,q_0^2 + 20\,q_2 - 8\right)q_1}{2} - \frac{9\,q_0^2\,t_0\,t_1}{2} + 3\,q_3\,t_0^2 + 3\,q_2\,t_0\,t_1 + 5\,q_0\,q_3 - q_5$$

$$EL4z := \frac{\left(-3\,q_0^2 + 2\,q_2\right)t_0^3}{2} + \frac{\left(-6\,q_0^3 + \left(22\,q_2 - 4\right)q_0 + 18\,q_1^2 - 6\,q_4\right)t_0}{2} + \frac{3\,q_0^2\,t_2}{2} + 9\,t_1\,q_0\,q_1 - q_2\,t_2 - 3\,t_1\,q_3 \quad \textbf{(4.21)}$$

> $solve([EL4y, EL4z], [q[5], q[4]])[1]$

$$\left[q_5 = -\frac{9}{2}\,q_0^2\,t_0\,t_1 - 9\,q_0\,q_1\,t_0^2 + 3\,q_2\,t_0\,t_1 + 3\,q_3\,t_0^2 - \frac{15}{2}\,q_0^2\,q_1 + 5\,q_0\,q_3 + 10\,q_2\,q_1 - 4\,q_1,\ q_4 = -\frac{1}{6\,t_0}\left(3\,q_0^2\,t_0^3 + 6\,q_0^3\,t_0 - 2\,q_2\,t_0^3 - 3\,q_0^2\,t_2 - 18\,t_1\,q_0\,q_1 - 22\,q_2\,t_0\,q_0 - 18\,q_1^2\,t_0 + 4\,t_0\,q_0 + 2\,q_2\,t_2 + 6\,t_1\,q_3\right)\right] \quad \textbf{(4.22)}$$

**Global invariant Lagrangian example:**

Lagrangian = T[0]^-1 T[1]^-1 omega, Eulerian = -2 t[0]^-2 t[1]^-1 - 2 t[2] t[0]^-1 t[1]^-3 , Hamiltonian = -2 t[0]^-1 t[1]^-1

> $EL5y := simplify\left(eval\left(ATystar, \left[seq\left(f[l] = TotalDiff\left(-\frac{2}{t[0]^2\,t[1]} - \frac{2\,t[2]}{t[0]\,t[1]^3}, [l]\right), l = 0..5\right)\right]\right) + eval\left(Bystar, \left[seq\left(f[l] = TotalDiff\left(-\frac{2}{t[0]\,t[1]}, [l]\right), l = 0..5\right)\right]\right)\right) :$
> $EL5z := simplify\left(eval\left(ATzstar, \left[seq\left(f[l] = TotalDiff\left(-\frac{2}{t[0]^2\,t[1]} - \frac{2\,t[2]}{t[0]\,t[1]^3}, [l]\right), l = 0..5\right)\right]\right) + eval\left(Bzstar, \left[seq\left(f[l] = TotalDiff\left(-\frac{2}{t[0]\,t[1]}, [l]\right), l = 0..5\right)\right]\right)\right) :$

> *solve*([EL5y, EL5z], [t[5], t[4]])[1] :

We express these conformally invariant EL in terms of the global invariants:

> *DGsetup*([s], [t, q, P, R, f], H) : # t = T, q = Q, II, JJ are global invariants

> *Nabla* := f → t[0]·t[1]· *TotalDiff*(f, [1])
 # global invariant derivation (TotalDiff is wrt Domega)

$$\nabla := f \mapsto t_0 \cdot t_1 \cdot TotalDiff(f, [1]) \quad \textbf{(4.23)}$$

> *nablatoomega* := [P[0] = t[0]^4, R[0] = q[0] t[0]^2] :
**for** i **from** 1 **to** 8 **do**:
*nablatoomega* := *simplify*([*op*(*nablatoomega*), P[i] = *Nabla*(*rhs*(*nablatoomega*[−2])), R[i] = *Nabla*(*rhs*(*nablatoomega*[−1]))], *symbolic*) :
**end do**: *nablatoomega*[1..15] :

> *localtoglobal_sub* := *simplify*(*solve*(*nablatoomega*[1..13], [t[6], q[5], t[5], q[4], t[4], q[3], t[3], q[2], t[2], q[1], t[1], q[0], t[0]]), *symbolic*)[1] :

> *simplify*(*eval*([EL5y, EL5z], *localtoglobal_sub*), *symbolic*)

$$\Bigg[\frac{1}{P_0^2 P_1^7}\Bigg(5 P_1^8 - 12 P_0^2 P_1^7 + \left(-8 P_0^2 R_1 - 20 P_0 P_2\right) P_1^6 + \Big(28 P_0^3 P_2 + \big(-16 P_2 R_0 + 306 P_3\big) P_0^2\Big) P_1^5 + 8\left(P_0^2 P_3 + \left(P_2 R_1 - 2 R_0 P_3 + 82 P_4\right) P_0 - \frac{327 P_2^2}{4}\right) P_0^2 P_1^4 - 20\Bigg(\Big(P_2^2 - 8 P_5\Big) P_0 - 2 R_0 P_2^2 + \frac{1217 P_2 P_3}{5}\Bigg) P_0^3 P_1^3 + \Big(\big(-1840 P_2 P_4 - 1280 P_3^2\big) P_0^4 + 5748 P_0^3 P_2^3\Big) P_1^2 + 10560 P_0^4 P_1 P_2^2 P_3 - 8800 P_0^4 P_2^4\Bigg),$$

$$\frac{1}{P_0^3 P_1^8 RootOf\left(4\_Z^2 P_0 - P_1\right)}\Bigg(2\, RootOf\left(\_Z^4 - P_0\right)^2 \Bigg(-\frac{5 P_0 P_1^9}{4} + \Bigg(-P_0^3 + \left(-1 - 2 R_0\right) P_0^2 - \frac{25 P_2}{4}\Bigg) P_1^8 + \frac{P_0\left(P_0 P_2 + 70 P_3\right) P_1^7}{4} + \Bigg(P_0^3 P_2 + \Big(\left(2 R_0 + 2\right) P_2 + 24 P_3\Big) P_0^2 + \left(10 P_2 R_1 + 36 R_0 P_3 - 146 P_4\right) P_0 - \frac{125 P_2^2}{4}\Bigg) P_0 P_1^6 + 12 P_0^2 \Bigg(P_0^2 P_4 + \left(\frac{4 R_0 P_4}{3} - \frac{14 P_2^2}{3} + \frac{2 P_3 R_1}{3} - \frac{46 P_5}{3}\right) P_0 - \frac{20 R_0 P_2^2}{3} + \frac{509 P_2 P_3}{6}\Bigg) P_1^5 - 96\Bigg(\left(P_2 P_3 + \frac{P_6}{3}\right) P_0^2 + \left(\frac{5 P_2^2 R_1}{24} + \left(\frac{4 R_0 P_3}{3} - \frac{493 P_4}{24}\right) P_2 - \frac{29 P_3^2}{2}\right) P_0 + \frac{765 P_2^3}{64}\Bigg) P_0^2 P_1^4 + \Big(\left(120 P_2^3 + 496 P_2 P_5 + 880 P_3 P_4\right) P_0^4 + \big(160 R_0 P_2^3 - 10802$$

**(4.24)**

$P_2^2 P_3) P_0^3) P_1^3 + ((-3952 P_2^2 P_4 - 5504 P_2 P_3^2) P_0^4 + 8630 P_0^3 P_2^4) P_1^2 + 19712 P_0^4 P_1 P_2^3 P_3$

$- 12320 P_0^4 P_2^5)))]$

global invariant EL for Lagrangian T^-1 T_omega^-1 omega in terms of global invariants:

> $EQ := solve(simplify(eval([EL5y, EL5z], localtoglobal\_sub), symbolic), [P[6], P[5]])[1]$

$$EQ := \Big[P_6 = \frac{1}{640 P_0^5 P_1^4} (20 P_0^5 P_1^6 P_2 - 20 P_0^4 P_1^8 + 40 P_0^4 P_1^6 P_2 R_0 - 40 P_0^3 P_1^8 R_0 + 240 P_0^5 P_1^5 P_4 - 2416 P_0^5 P_1^4 P_2 P_3 + 3640 P_0^5 P_1^3 P_2^3 + 40 P_0^4 P_1^6 P_2 + 664 P_0^4 P_1^6 P_3 - 3316 P_0^4 P_1^5 P_2^2 + 160 P_0^4 P_1^5 P_3 R_1 + 320 P_0^4 P_1^5 P_4 R_0 - 896 P_0^4 P_1^4 P_2^2 R_1 - 1568 P_0^4 P_1^4 P_2 P_3 R_0 + 720 P_0^4 P_1^3 P_2^3 R_0 - 20 P_0^3 P_1^8 + 1393 P_0^3 P_1^7 P_2 + 880 P_0^3 P_1^6 P_2 R_1 + 352 P_0^3 P_1^6 P_3 R_0 + 312 P_0^3 P_1^5 P_2^2 R_0 - 301 P_0^2 P_1^9 - 184 P_0^2 P_1^8 R_1 - 368 P_0^2 P_1^7 P_2 R_0 + 17600 P_0^5 P_1^3 P_3 P_4 + 35040 P_0^5 P_1^2 P_2^2 P_4 - 30720 P_0^5 P_1^2 P_2 P_3^2 - 260480 P_0^5 P_1 P_2^3 P_3 + 299200 P_0^5 P_2^5 - 43552 P_0^4 P_1^4 P_2 P_4 - 1600 P_0^4 P_1^4 P_3^2 + 328656 P_0^4 P_1^3 P_2^2 P_3 - 386176 P_0^4 P_1^2 P_2^4 + 12168 P_0^3 P_1^6 P_4 - 110576 P_0^3 P_1^5 P_2 P_3 + 149802 P_0^3 P_1^4 P_2^3 + 7388 P_0^2 P_1^7 P_3 - 14427 P_0^2 P_1^6 P_2^2 - 895 P_0 P_1^8 P_2 + 115 P_1^{10}), P_5 = -\frac{1}{160 P_1^3 P_0^4} (8 P_0^4 P_1^4 P_3 - 20 P_0^4 P_1^3 P_2^2 + 28 P_0^3 P_1^5 P_2 + 8 P_0^3 P_1^4 P_2 R_1 - 16 P_0^3 P_1^4 P_3 R_0 + 40 P_0^3 P_1^3 P_2^2 R_0 - 12 P_0^2 P_1^7 - 8 P_0^2 P_1^6 R_1 - 16 P_0^2 P_1^5 P_2 R_0 - 1840 P_0^4 P_1^2 P_2 P_4 - 1280 P_0^4 P_1^2 P_3^2 + 10560 P_0^4 P_1 P_2^2 P_3 - 8800 P_0^4 P_2^4 + 656 P_0^3 P_1^4 P_4 - 4868 P_0^3 P_1^3 P_2 P_3 + 5748 P_0^3 P_1^2 P_2^3 + 306 P_0^2 P_1^5 P_3 - 654 P_0^2 P_1^4 P_2^2 - 20 P_0 P_1^6 P_2 + 5 P_1^8)\Big] \quad \textbf{(4.25)}$$

> $tmp5 := eval(TotalDiff(EQ[2], 1), EQ) : tmp4 := solve\big(lhs(tmp5) - rhs(tmp5), \{P_4\}\big) :$

> $solve\big(\{EQ[2], tmp4[1]\}, \{P_5, R_2\}\big)$

$$\Big\{P_5 = -\frac{1}{160 P_1^3 P_0^4} (8 P_0^4 P_1^4 P_3 - 20 P_0^4 P_1^3 P_2^2 + 28 P_0^3 P_1^5 P_2 + 8 P_0^3 P_1^4 P_2 R_1 - 16 P_0^3 P_1^4 P_3 R_0 \quad \textbf{(4.26)}$$

$$+ 40 P_0^3 P_1^3 P_2^2 R_0 - 12 P_0^2 P_1^7 - 8 P_0^2 P_1^6 R_1 - 16 P_0^2 P_1^5 P_2 R_0 - 1840 P_0^4 P_1^2 P_2 P_4 - 1280 P_0^4 P_1^2 P_3^2 + 10560 P_0^4 P_1 P_2^2 P_3 - 8800 P_0^4 P_2^4 + 656 P_0^3 P_1^4 P_4 - 4868 P_0^3 P_1^3 P_2 P_3 + 5748 P_0^3 P_1^2 P_2^3 + 306 P_0^2 P_1^5 P_3 - 654 P_0^2 P_1^4 P_2^2 - 20 P_0 P_1^6 P_2 + 5 P_1^8\Big), R_2 =$$

$$-\frac{1}{160 P_0^3 P_1^3 \left(P_0 P_2 - P_1^2\right)} \Big(100 P_0^5 P_1^4 P_2 - 100 P_0^4 P_1^6 + 200 P_0^4 P_1^4 P_2 R_0 - 200 P_0^3 P_1^6 R_0 + 1360 P_0^5 P_1^3 P_4 - 10880 P_0^5 P_1^2 P_2 P_3 + 13600 P_0^5 P_1 P_2^3 + 200 P_0^4 P_1^4 P_2 + 3224 P_0^4 P_1^4 P_3 - 7380 P_0^4 P_1^3 P_2^2 + 640 P_0^4 P_1^3 P_3 R_1 + 1280 P_0^4 P_1^3 P_4 R_0 - 1680 P_0^4 P_1^2 P_2^2 R_1 - 10240 P_0^4 P_1^2 P_2 P_3 R_0 + 12800 P_0^4 P_1 P_2^3 R_0 - 100 P_0^3 P_1^6 + 389 P_0^3 P_1^5 P_2 + 944 P_0^3 P_1^4 P_2 R_1 + 3072 P_0^3 P_1^4 P_3 R_0 - 6840 P_0^3 P_1^3 P_2^2 R_0 - 41 P_0^2 P_1^7 + 56 P_0^2 P_1^6 R_1 + 112 P_0^2 P_1^5 P_2 R_0 - 240 P_0^4 P_1^2 P_2 P_4 - 400 P_0^4 P_1^2 P_3^2 + 2600 P_0^4 P_1 P_2^2 P_3 - 2200 P_0^4 P_2^4 + 48 P_0^3 P_1^4 P_4 + 116 P_0^3 P_1^3 P_2 P_3 - 786 P_0^3 P_1^2 P_2^3 - 792 P_0^2 P_1^5 P_3 + 1853 P_0^2 P_1^4 P_2^2 + 15 P_0 P_1^6 P_2 - 235 P_1^8\Big)\}$$

## Computing W:

```
> DGsetup([x], [y, z], E, 12) :
> omega := evalDG(1/Domega(x) dx) : # omega, conformal arclength parameter
> vartheta1 := evalDG(2/Domega(x)^5 (diff(Q, y[5])·(dy[0] − y[1] dx) + diff(Q, z[5])
    ·(dz[0] − z[1] dx) )) : vartheta2 := evalDG(1/Domega(x)^4 (diff(T, y[4])·(dy[0]
    − y[1] dx) + diff(T, z[4])·(dz[0] − z[1] dx) )) :
    # invariant contact forms of order 0 constructed from the symbols of the differential invariants
    T,Q
> eval([vartheta1, vartheta2], cs)
    # conclusion: vartheta1 = iota(theta_y0), vartheta2 = iota(theta_z0)
```

$$[0\,dx + dy_0 + 0\,dz_0,\ 0\,dx + 0\,dy_0 + dz_0] \quad \textbf{(4.3.1)}$$

```
> solve(DGinfo(evalDG(vartheta1 &w omega − W1y·(dy[0]−y[1]·dx) &w dx − W1z ·(dz[0]
    −z[1]·dx) &w dx), "CoefficientSet") union DGinfo(evalDG(vartheta2 &w omega − W2y
    ·(dy[0]−y[1]·dx) &w dx − W2z·(dz[0]−z[1]·dx) &w dx), "CoefficientSet"), [W1y,
    W1z, W2y, W2z])[1] : W := simplify(eval(Matrix([[W1y, W1z], [W2y, W2z]]), %),
    symbolic)
```

$W :=$ **(4.3.2)**

$$\left[\begin{array}{c}\frac{y_3 z_1^4 + \left(-y_1 z_3 - 3 y_2 z_2\right) z_1^3 + \left(y_1^2 y_3 + \left(-3 y_2^2 + 3 z_2^2\right) y_1 + 2 y_3\right) z_1^2 + \left(-y_1^3 z_3\right.}{\left(y_1^2 + z_1^2 + 1\right)^3} \cdots \\ -\frac{z_3 \left(y_1^2 + z_1^2 + 1\right) - 3 y_1 z_2 y_2 -}{\left(y_1^2 + z_1^2 + 1\right)^{5/2}} \cdots\end{array}\right]$$

> *solve*( [ *W*[1, 2], *W*[2, 2]], [*y*[3], *z*[3]]) [1] # *unparametrized conformal geodesic equations*

$$\left[y_3 = \frac{3 y_2 \left(y_1 y_2 + z_1 z_2\right)}{y_1^2 + z_1^2 + 1}, z_3 = \frac{3 \left(y_1 y_2 + z_1 z_2\right) z_2}{y_1^2 + z_1^2 + 1}\right] \quad \textbf{(4.3.3)}$$

>

>

**Conclusion:** For the conformal torsion functional T omega, we got that E_inv(T) = [0,-1]^T. Setting this equal to zero gives no regular solutions. The ordinary EL equations are obtained by multiplying the matrix relative invariant W with the invariant EL vector [0,-1]^T. We computed this above and solved for third-jets to obtain the (unparametrized) conformal geodesic equations.

>

# Euclidean 4D

> *restart* : *with*(*DifferentialGeometry*) : *with*(*LieAlgebras*) : *with*(*Tensor*) : *with*(*GroupActions*) : *with*(*Tools*) : *Preferences*("ShowFramePrompt",'*false*') : *interface*(*warnlevel* = 0) : *with*(*LinearAlgebra*) : *with*(*PDETools*) : *with*(*JetCalculus*) : *with*(*ArrayTools*) : *Preferences*("JetNotation", "JetNotation2") :

> *DGsetup*([*x*], [*y*, *z*, *u*], *E*, 12) : *totalD* := *evalDG*(*D_x* + *add*(*y*[*i* + 1] *D_y*[*i*], *i* = 0 ..10 ) + *add*(*z*[*i* + 1] *D_z*[*i*], *i* = 0 ..10 ) + *add*(*u*[*i* + 1] *D_u*[*i*], *i* = 0 ..10 )) : *contact_forms* := [*seq*(*op*([*dy*[*i*] − *y*[*i* + 1] *dx*, *dz*[*i*] − *z*[*i* + 1] *dx*, *du*[*i*] − *u*[*i* + 1] *dx*]), *i* = 0 ..8)] :

**Lie algebra of Euclidean group:**

> *iso* := *evalDG*([*D_x*, *D_y*[0], *D_z*[0], *D_u*[0], *x D_y*[0] − *y*[0] *D_x*, *x D_z*[0] − *z*[0] *D_x*, *x D_u*[0] − *u*[0] *D_x*, *y*[0] *D_z*[0] − *z*[0] *D_y*[0], *y*[0] *D_u*[0] − *u*[0] *D_y*[0], *z*[0] *D_u*[0] − *u*[0] *D_z*[0]]) : *g* := *map*(*Prolong*, *iso*, 5) : *r* := *nops*(*g*)

$$r := 10 \quad \textbf{(5.1)}$$

**Local invariants and invariant derivation:**

We have differential invariants kappa, tau, mu of orders 2,3,4, respectively.

> kappa := $\frac{1}{\left(1 + y[1]^2 + z[1]^2 + u[1]^2\right)^{\frac{3}{2}}} \left(\mathrm{sqrt}\left((y[1] z[2] - y[2] z[1])^2 + (y[1] u[2] - y[2] u[1])^2 + (u[1] z[2] - u[2] z[1])^2 + y[2]^2 + z[2]^2 + u[2]^2\right)\right)$

$$\kappa := \frac{\sqrt{\left(y_1 z_2 - y_2 z_1\right)^2 + \left(-y_2 u_1 + y_1 u_2\right)^2 + \left(u_1 z_2 - u_2 z_1\right)^2 + y_2^2 + z_2^2 + u_2^2}}{\left(u_1^2 + y_1^2 + z_1^2 + 1\right)^{3/2}} \quad \textbf{(5.2)}$$

> tau := $\left(\mathrm{sqrt}\left(\mathit{Determinant}\left(\mathit{Matrix}([[y[1], z[1], u[1]], [y[2], z[2], u[2]], [y[3], z[3], u[3]]])\right)\right)^2$

$$+ (y[2]z[3] - z[2]y[3])^2 + (y[2]u[3] - u[2]y[3])^2 + (u[2]z[3] - z[2]u[3])^2) \Big) \Big/ \Big( (y[1]z[2] - z[1]y[2])^2 + (y[1]u[2] - u[1]y[2])^2 + (u[1]z[2] - z[1]u[2])^2 + y[2]^2 + z[2]^2 + u[2]^2 \Big)$$

$$\tau := \Big( (u_1 y_2 z_3 - u_1 y_3 z_2 - u_2 y_1 z_3 + u_2 y_3 z_1 + u_3 y_1 z_2 - u_3 y_2 z_1)^2 + (y_2 z_3 - z_2 y_3)^2 + (-u_2 y_3 + y_2 u_3)^2 + (u_2 z_3 - z_2 u_3)^2 \Big)^{1/2} \Big/ \Big( (y_1 z_2 - z_1 y_2)^2 + (-u_1 y_2 + y_1 u_2)^2 + (u_1 z_2 - z_1 u_2)^2 + y_2^2 + z_2^2 + u_2^2 \Big) \quad (5.3)$$

> $\mathrm{mu} := \dfrac{Determinant(Matrix([[y[2], z[2], u[2]], [y[3], z[3], u[3]], [y[4], z[4], u[4]]]))}{(1 + y[1]^2 + z[1]^2 + u[1]^2)^5} \cdot (\kappa^3 \tau^2)^{-1}$

$$\mu := \Big( (u_2 y_3 z_4 - u_2 y_4 z_3 - u_3 y_2 z_4 + u_3 y_4 z_2 + u_4 y_2 z_3 - u_4 y_3 z_2) \sqrt{(y_1 z_2 - y_2 z_1)^2 + (-u_1 y_2 + u_2 y_1)^2 + (u_1 z_2 - u_2 z_1)^2 + y_2^2 + z_2^2 + u_2^2} \Big) \Big/ \Big( \sqrt{u_1^2 + y_1^2 + z_1^2 + 1} \, \big( (u_1 y_2 z_3 - u_1 y_3 z_2 - u_2 y_1 z_3 + u_2 y_3 z_1 + u_3 y_1 z_2 - u_3 y_2 z_1)^2 + (y_2 z_3 - y_3 z_2)^2 + (-u_2 y_3 + u_3 y_2)^2 + (u_2 z_3 - u_3 z_2)^2 \big) \Big) \quad (5.4)$$

> $Ts := f \rightarrow simplify\left( \dfrac{1}{\mathrm{sqrt}(1 + y[1]^2 + z[1]^2 + u[1]^2)} \cdot TotalDiff(f, x),\ symbolic \right):$

> $\kappa0 := \kappa$ :**for** $i$ **to** 2 **do** $\kappa \| i := Ts(\kappa \| (i-1))$:**od**: $\tau0 := \tau$ :**for** $i$ **to** 1 **do** $\tau \| i := Ts(\tau \| (i-1))$:**od**:

> $cs0 := [x = 0, y[0] = 0, y[1] = 0, z[0] = 0, z[1] = 0, z[2] = 0, u[0] = 0, u[1] = 0, u[2] = 0, u[3] = 0]:$

> $invariantizations := solve(simplify(eval([\mathrm{kappa} = K, \mathrm{tau} = T, \mathrm{mu} = M, kappa1 = K1, tau1 = T1, kappa2 = K2], cs0), symbolic), [y[2], y[3], y[4], z[3], z[4], u[4]])[1]$

$$invariantizations := [y_2 = K, y_3 = K1, y_4 = 3K^3 - K T^2 + K2, z_3 = K T, z_4 = K T1 + 2 K1 T, u_4 = K M T] \quad (5.5)$$

We update cross-section to include invariantizations:

> $cs := [op(cs0), op(invariantizations), d\_x = \mathrm{varpi}]$

$$cs := [x = 0, y_0 = 0, y_1 = 0, z_0 = 0, z_1 = 0, z_2 = 0, u_0 = 0, u_1 = 0, u_2 = 0, u_3 = 0, y_2 = K, y_3 = K1, y_4 = 3K^3 - K T^2 + K2, z_3 = K T, z_4 = K T1 + 2 K1 T, u_4 = K M T, d\_x = \varpi] \quad (5.6)$$

**Step 1: Defining horizontal and vertical derivative, horizontal and vertical component of a one-form on J^infinity, as well as iota composed with dV and vertpart.**

```
> horpart := eta → Hook(totalD, eta) · d_x :
      # horizontal part of a one-form (NB: d_x is a symbol!)
  vertpart := eta→ add(Hook(D_y[i], eta) · cat(theta_y, i) + Hook(D_z[i], eta) · cat(theta_z, i)
      + Hook(D_u[i], eta) · cat(theta_u, i), i = 0 ..12) : # vertical part of a one-form
  dH := f→ Hook(totalD, ExteriorDerivative(f) ) · d_x : # horizontal derivative of a function
  dV := f→ vertpart(VerticalExteriorDerivative(f) ) : # vertical derivative of a function
```

```
iotavertpart := eta→ add(eval(Hook(D_y[i], eta), cs)·cat(iota_theta_y, i)
    + eval(Hook(D_z[i], eta), cs)·cat(iota_theta_z, i) + eval(Hook(D_u[i], eta), cs)
    ·cat(iota_theta_u, i), i = 0..12) : # iota composed with vertical part of one-form
iotadV := f→ add(eval(Hook(D_y[i], ExteriorDerivative(f), cs)·cat(iota_theta_y, i)
    + Hook(D_z[i], ExteriorDerivative(f), cs)·cat(iota_theta_z, i) + Hook(D_u[i],
    ExteriorDerivative(f), cs)·cat(iota_theta_u, i)   ), i = 0..10) : # iota composed with dV
```

**Step 2: Computing gamma and epsilon terms**

```
> csvars := map(lhs, cs0) : # jet variables that are constant on the cross-section
> for j from 1 to r do;
  gam || j := eval(dH(csvars[j]) + add(LieDerivative(g[i], csvars[j])·gamma[i], i = 1..r),
      cs) :
  end do:
  gammas := solve([seq(gam || j = 0, j = 1..r)], [seq(gamma[j], j = 1..r)])[1]
```

$$gammas := [\gamma_1 = -\varpi, \gamma_2 = 0, \gamma_3 = 0, \gamma_4 = 0, \gamma_5 = -K\,\varpi, \gamma_6 = 0, \gamma_7 = 0, \gamma_8 = -T\,\varpi, \gamma_9 = 0, \gamma_{10} = -M\,\varpi] \tag{5.7}$$

```
> for j from 1 to r do;
  eps || j := iotadV(csvars[j]) + eval(add(LieDerivative(g[i], csvars[j]·epsilon[i]), i = 1..r),
      cs) :
  end do:
  epsilons := solve([seq(eps || j = 0, j = 1..r)], [seq(epsilon[j], j = 1..r )])[1]
```

$$epsilons := \left[\epsilon_1 = 0, \epsilon_2 = -iota\_theta\_y0, \epsilon_3 = -iota\_theta\_z0, \epsilon_4 = -iota\_theta\_u0, \epsilon_5 = -iota\_theta\_y1, \epsilon_6 = -iota\_theta\_z1, \epsilon_7 = -iota\_theta\_u1, \epsilon_8 = -\frac{iota\_theta\_z2}{K}, \epsilon_9 = -\frac{iota\_theta\_u2}{K}, \epsilon_{10} = -\frac{K\,iota\_theta\_u3 - K1\,iota\_theta\_u2}{K^2\,T}\right] \tag{5.8}$$

**Step 3: Computing invariant vertical derivatives of curvatures kappa, tau, mu:**

```
> dvkappa := simplify(eval(iotadV(kappa) + eval(add(LieDerivative(g[i], kappa)·epsilon[i],
      i = 1..r), epsilons), cs), symbolic)
```

$$dvkappa := iota\_theta\_y2 \tag{5.9}$$

```
> dvtau := simplify(eval(iotadV(tau) + eval(add(LieDerivative(g[i], tau)·epsilon[i], i = 1
      ..r), epsilons), cs), symbolic)
```

$$dvtau := \frac{(-T\,iota\_theta\_y2 + iota\_theta\_z3)\,K - K1\,iota\_theta\_z2}{K^2} \tag{5.10}$$

```
> dvmu := expand(simplify(eval(iotadV(mu) + eval(add(LieDerivative(g[i], mu)·epsilon[i], i
      = 1..r), epsilons), cs), symbolic))
```

$$dvmu := -\frac{3\,K\,iota\_theta\_u2}{T} + \frac{T\,iota\_theta\_u2}{K} - \frac{M\,iota\_theta\_z3}{K\,T} + \frac{M\,K1\,iota\_theta\_z2}{K^2\,T} + \frac{iota\_theta\_u4}{K\,T} - \frac{T1\,iota\_theta\_u3}{K\,T^2} - \frac{2\,K1\,iota\_theta\_u3}{K^2\,T} + \frac{K1\,T1\,iota\_theta\_u2}{K^2\,T^2} - \frac{K2\,iota\_theta\_u2}{K^2\,T} + \frac{2\,K1^2\,iota\_theta\_u2}{K^3\,T} \tag{5.11}$$

**Computing invariant vertical derivative of ϖ:**
Here we actually compute the invariant contact form B where d_V(varpi) = B wedge varpi. (Substituting varpi = 1 amounts to hooking with invariant derivation D_s. Note minus sign.)

```
> B := eval(eval(eval(add(epsilon[i] · horpart(LieDerivative(g[i], dx)) − gamma[i]
      · iotavertpart(LieDerivative(g[i], dx)), i = 1..r), [op(epsilons), op(gammas)]), cs),
      [varpi = 1])
```

$$B := -K\ iota\_theta\_y0 \qquad (5.12)$$

**Steps 4-5: Computing the correction terms in ι(θ_i+1) = D_omega(ι(θ_i)) + corrterm_i+1.**

```
> sub := [K = K[0], K1 = K[1], K2 = K[2], T = T[0], T1 = T[1], M = M[0], M1 = M[1],
      seq(iota_theta_y||i = ICy||i[0], i = 0..4), seq(iota_theta_z||i = ICz||i[0], i = 0..4),
      seq(iota_theta_u||i = ICu||i[0], i = 0..4) ]
```

$$sub := [K = K_0, K1 = K_1, K2 = K_2, T = T_0, T1 = T_1, M = M_0, M1 = M_1, iota\_theta\_y0 = ICy0_0, iota\_theta\_y1 = ICy1_0, iota\_theta\_y2 = ICy2_0, iota\_theta\_y3 = ICy3_0, iota\_theta\_y4 = ICy4_0, iota\_theta\_z0 = ICz0_0, iota\_theta\_z1 = ICz1_0, iota\_theta\_z2 = ICz2_0, iota\_theta\_z3 = ICz3_0, iota\_theta\_z4 = ICz4_0, iota\_theta\_u0 = ICu0_0, iota\_theta\_u1 = ICu1_0, iota\_theta\_u2 = ICu2_0, iota\_theta\_u3 = ICu3_0, iota\_theta\_u4 = ICu4_0] \qquad (5.1.1)$$

Computing the correction terms:

```
> for j from 1 to 15 do;
  corrterm||j := eval(eval(eval(eval(horpart(add(gamma[i] LieDerivative(g[i],
      contact_forms[j]), i = 1..r)) + add(Hook(D_y[l], (add(gamma[i] LieDerivative(g[i],
      contact_forms[j]), i = 1..r)))·iota_theta_y||l, l = 0..10) + add(Hook(D_z[l],
      (add(gamma[i] LieDerivative(g[i], contact_forms[j]), i = 1..r)))·iota_theta_z||l, l = 0
      ..10) + add(Hook(D_u[l], (add(gamma[i] LieDerivative(g[i], contact_forms[j]), i = 1
      ..r)))·iota_theta_u||l, l = 0..10), [op(epsilons), op(gammas)]), cs), [varpi = 1]), sub)
  end do :
> DGsetup([s], [K, T, M, seq(ICy||i, i = 0..4), seq(ICz||i, i = 0..4), seq(ICu||i, i = 0..4), f], G,
      5) :
```

We express invariant contact forms IC||i[0] as a differential operator acting on IC0[0]'s:

```
> ICforms := [seq(op([ICy||i[0], ICz||i[0], ICu||i[0]]), i = 1..4)] :
> eq1 := ICy1[0] = ICy0[1] − corrterm1 : eq := [eq1] :
  eq2 := ICz1[0] = ICz0[1] − corrterm2 : eq := [op(eq), eq2] :
  eq3 := ICu1[0] = ICu0[1] − corrterm3 : eq := [op(eq), eq3] :
  for i from 4 to 12 do: j := i − 1 :
  eq||i := ICforms[i] = eval(TotalDiff(eval(ICforms[i − 3], eq), 1) −corrterm||i, eq) ; eq :=
      [op(eq), eq||i] :
  end do:
> expand(eq4) # example
```

$$ICy2_0 = ICu0_0\, M_0\, T_0 + ICy0_0\, K_0^2 - ICy0_0\, T_0^2 - ICz0_0\, T_1 - 2\, T_0\, ICz0_1 + ICy0_2 \qquad (5.1.2)$$

**Step 6: Collecting differential operators from dvq, B**

```
> DGsetup([s], [K, T, M, seq(ICy||i, i = 0..4), seq(ICz||i, i = 0..4), seq(ICu||i, i = 0..4), f],
      G, 5) :
> dvkappanew := expand(eval(eval(dvkappa , sub), eq));
```

$dvtaunew := expand(eval(eval(dvtau, sub), eq));$

$dvmunew := expand(eval(eval(dvmu, sub), eq))$

$$dvkappanew := ICu0_0\,M_0\,T_0 + ICy0_0\,K_0^2 - ICy0_0\,T_0^2 - ICz0_0\,T_1 - 2\,T_0\,ICz0_1 + ICy0_2$$

$$dvtaunew := -K_0\,ICu0_0\,M_0 + \frac{ICu0_0\,M_0^3}{K_0} + 2\,ICy0_0\,K_0\,T_0 - \frac{ICy0_0\,M_0^2\,T_0}{K_0} - \frac{3\,ICz0_0\,M_0\,M_1}{K_0} - \frac{2\,ICz0_0\,T_0\,T_1}{K_0} + \frac{ICz0_0\,K_1\,M_0^2}{K_0^2} + \frac{ICz0_0\,K_1\,T_0^2}{K_0^2} + K_0\,ICz0_1 - \frac{3\,ICz0_1\,M_0^2}{K_0} - \frac{ICz0_1\,T_0^2}{K_0} - \frac{ICu0_0\,M_2}{K_0} + \frac{ICu0_0\,K_1\,M_1}{K_0^2} - \frac{3\,ICu0_1\,M_1}{K_0} + \frac{2\,ICu0_1\,K_1\,M_0}{K_0^2} - \frac{3\,ICu0_2\,M_0}{K_0} + \frac{ICy0_0\,T_2}{K_0} - \frac{ICy0_0\,K_1\,T_1}{K_0^2} + \frac{3\,ICy0_1\,T_1}{K_0} - \frac{2\,ICy0_1\,K_1\,T_0}{K_0^2} + \frac{2\,ICy0_2\,T_0}{K_0} - \frac{ICz0_2\,K_1}{K_0^2} + \frac{ICz0_3}{K_0}$$

$$dvmunew := -\frac{3\,M_0^2\,ICu0_2}{K_0\,T_0} + \frac{3\,M_0\,ICy0_2}{K_0} + \frac{3\,M_0\,ICz0_3}{K_0\,T_0} - \frac{3\,ICu0_0\,M_1^2}{K_0\,T_0} + \frac{ICu0_1\,K_1}{T_0} + \frac{ICy0_0\,M_2}{K_0} + \frac{4\,ICy0_1\,M_1}{K_0} + \frac{ICz0_0\,M_3}{K_0\,T_0} + \frac{4\,ICz0_1\,M_2}{K_0\,T_0} + \frac{6\,M_1\,ICz0_2}{K_0\,T_0} - \frac{K_0\,T_1\,ICu0_1}{T_0^2} - \frac{T_1\,ICu0_3}{K_0\,T_0^2} - \frac{2\,K_1\,ICu0_3}{K_0^2\,T_0} - \frac{K_2\,ICu0_2}{K_0^2\,T_0} + \frac{2\,K_1^2\,ICu0_2}{K_0^3\,T_0} - \frac{3\,M_0^2\,ICz0_0\,M_1}{K_0\,T_0} - \frac{M_0\,ICz0_0\,T_1}{K_0} - \frac{3\,M_0\,ICu0_0\,M_2}{K_0\,T_0} - \frac{9\,M_0\,M_1\,ICu0_1}{K_0\,T_0} + \frac{2\,M_0\,ICy0_0\,T_2}{K_0\,T_0} + \frac{2\,M_0\,T_1\,ICy0_1}{K_0\,T_0} + \frac{M_0^3\,K_1\,ICz0_0}{K_0^2\,T_0} + \frac{M_0\,T_0\,K_1\,ICz0_0}{K_0^2} + \frac{4\,M_0^2\,K_1\,ICu0_1}{K_0^2\,T_0} - \frac{4\,M_0\,K_1\,ICy0_1}{K_0^2} - \frac{5\,M_0\,K_1\,ICz0_2}{K_0^2\,T_0} + \frac{ICz0_0\,K_1\,M_0}{T_0} + \frac{2\,ICy0_0\,M_1\,T_1}{K_0\,T_0} - \frac{K_0\,T_1\,ICz0_0\,M_0}{T_0^2} + \frac{T_1\,ICz0_0\,M_0^3}{K_0\,T_0^2} + \frac{3\,T_1\,M_0^2\,ICu0_1}{K_0\,T_0^2} - \frac{2\,T_1^2\,M_0\,ICy0_0}{K_0\,T_0^2} - \frac{T_1\,ICz0_0\,M_2}{K_0\,T_0^2} - \frac{3\,T_1\,M_1\,ICz0_1}{K_0\,T_0^2} - \frac{3\,T_1\,M_0\,ICz0_2}{K_0\,T_0^2} - \frac{2\,K_1\,ICy0_0\,M_1}{K_0^2} - \frac{2\,K_1\,ICz0_0\,M_2}{K_0^2\,T_0} - \frac{6\,K_1\,M_1\,ICz0_1}{K_0^2\,T_0} + \frac{K_1\,T_1\,ICu0_2}{K_0^2\,T_0^2} + \frac{K_2\,ICu0_0\,M_0^2}{K_0^2\,T_0} - \frac{K_2\,ICy0_0\,M_0}{K_0^2} - \frac{K_2\,ICz0_0\,M_1}{K_0^2\,T_0} \tag{5.13}$$

$$- \frac{2 K_2 M_0 ICz0_1}{K_0^2 T_0} - \frac{2 K_1^2 ICu0_0 M_0^2}{K_0^3 T_0} + \frac{2 K_1^2 ICy0_0 M_0}{K_0^3} + \frac{2 K_1^2 ICz0_0 M_1}{K_0^3 T_0}$$
$$+ \frac{4 K_1^2 M_0 ICz0_1}{K_0^3 T_0} + K_0 ICy0_0 M_0 + \frac{K_0 ICz0_0 M_1}{T_0} + \frac{K_0 M_0 ICz0_1}{T_0} - \frac{T_0 ICu0_0 M_0^2}{K_0}$$
$$+ \frac{T_0^2 ICy0_0 M_0}{K_0} + \frac{T_0 M_0 ICz0_1}{K_0} - \frac{M_0^3 ICz0_1}{K_0 T_0} + \frac{5 M_0 K_1 ICu0_0 M_1}{K_0^2 T_0}$$
$$- \frac{2 M_0 K_1 ICy0_0 T_1}{K_0^2 T_0} + \frac{3 T_1 ICu0_0 M_0 M_1}{K_0 T_0^2} - \frac{K_1 T_1 ICu0_0 M_0^2}{K_0^2 T_0^2} + \frac{K_1 T_1 ICz0_0 M_1}{K_0^2 T_0^2}$$
$$+ \frac{2 K_1 T_1 M_0 ICz0_1}{K_0^2 T_0^2} + \frac{K_0 ICu0_2}{T_0} + \frac{ICu0_4}{K_0 T_0} + \frac{T_0 ICu0_2}{K_0}$$

**Collecting differential operators from**

> **for** *i* **from** 0 **to** 4 **do** $Aky \| i := coeff(dvkappanew, ICy0[i])$ **end do**: **for** *i* **from** 0 **to** 4 **do** $Akz \| i := coeff(dvkappanew, ICz0[i])$ **end do**:**for** *i* **from** 0 **to** 4 **do** $Aku \| i := coeff(dvkappanew, ICu0[i])$ **end do**:

> $simplify(dvkappanew - add(Aky \| i \; ICy0[i], i = 0 ..4) - add(Akz \| i \; ICz0[i], i = 0 ..4) - add(Aku \| i \; ICu0[i], i = 0 ..4))$

$$0 \qquad \textbf{(5.14)}$$

> **for** *i* **from** 0 **to** 4 **do** $Aty \| i := coeff(dvtaunew, ICy0[i])$ **end do**: **for** *i* **from** 0 **to** 4 **do** $Atz \| i := coeff(dvtaunew, ICz0[i])$ **end do**:**for** *i* **from** 0 **to** 4 **do** $Atu \| i := coeff(dvtaunew, ICu0[i])$ **end do**:

> $simplify(dvtaunew - add(Aty \| i \; ICy0[i], i = 0 ..4) - add(Atz \| i \; ICz0[i], i = 0 ..4) - add(Atu \| i \; ICu0[i], i = 0 ..4))$

$$0 \qquad \textbf{(5.15)}$$

> **for** *i* **from** 0 **to** 4 **do** $Amy \| i := coeff(dvmunew, ICy0[i])$ **end do**: **for** *i* **from** 0 **to** 4 **do** $Amz \| i := coeff(dvmunew, ICz0[i])$ **end do**: **for** *i* **from** 0 **to** 4 **do** $Amu \| i := coeff(dvmunew, ICu0[i])$ **end do**:

> $simplify(dvmunew - add(Amy \| i \; ICy0[i], i = 0 ..4) - add(Amz \| i \; ICz0[i], i = 0 ..4) - add(Amu \| i \; ICu0[i], i = 0 ..4))$

$$0 \qquad \textbf{(5.16)}$$

> $Aky := collect(expand(add(Aky \| j \; TotalDiff(ICy0[0], [j]), j = 0 ..4)), [seq(ICy0[i], i = 0 ..4), seq(ICz0[i], i = 0 ..4), seq(ICu0[i], i = 0 ..4)])$ :
$Akz := collect(expand(add(Akz \| j \; TotalDiff(ICz0[0], [j]), j = 0 ..4)), [seq(ICy0[i], i = 0 ..4), seq(ICz0[i], i = 0 ..4), seq(ICu0[i], i = 0 ..4)])$ :
$Aku := collect(expand(add(Aku \| j \; TotalDiff(ICu0[0], [j]), j = 0 ..4)), [seq(ICy0[i], i = 0 ..4), seq(ICz0[i], i = 0 ..4), seq(ICu0[i], i = 0 ..4)])$ :
$Aty := collect(expand(add(Aty \| j \; TotalDiff(ICy0[0], [j]), j = 0 ..4)), [seq(ICy0[i], i = 0 ..4), seq(ICz0[i], i = 0 ..4), seq(ICu0[i], i = 0 ..4)])$ :
$Atz := collect(expand(add(Atz \| j \; TotalDiff(ICz0[0], [j]), j = 0 ..4)), [seq(ICy0[i], i = 0 ..4), seq(ICz0[i], i = 0 ..4), seq(ICu0[i], i = 0 ..4)])$ :
$Atu := collect(expand(add(Atu \| j \; TotalDiff(ICu0[0], [j]), j = 0 ..4)), [seq(ICy0[i], i = 0 ..4), seq(ICz0[i], i = 0 ..4), seq(ICu0[i], i = 0 ..4)])$ :

$Amy := collect(expand(add(Amy \| j\ TotalDiff(ICy0[0], [j]), j = 0..4)), [seq(ICy0[i], i = 0..4), seq(ICz0[i], i = 0..4), seq(ICu0[i], i = 0..4)]):$

$Amz := collect(expand(add(Amz \| j\ TotalDiff(ICz0[0], [j]), j = 0..4)), [seq(ICy0[i], i = 0..4), seq(ICz0[i], i = 0..4), seq(ICu0[i], i = 0..4)]):$

$Amu := collect(expand(add(Amu \| j\ TotalDiff(ICu0[0], [j]), j = 0..4)), [seq(ICy0[i], i = 0..4), seq(ICz0[i], i = 0..4), seq(ICu0[i], i = 0..4)]):$

**Step 7: Computing formal adjoints**

> $Akystar := collect(expand(add(TotalDiff((-1)^j\ Aky \| j \cdot f[0], [j]), j = 0..4)), [f[4], f[3], f[2], f[1], f[0]]);$

$Akzstar := collect(expand(add(TotalDiff((-1)^j\ Akz \| j \cdot f[0], [j]), j = 0..4)), [f[4], f[3], f[2], f[1], f[0]]);$

$Akustar := collect(expand(add(TotalDiff((-1)^j\ Aku \| j \cdot f[0], [j]), j = 0..4)), [f[4], f[3], f[2], f[1], f[0]]);$

$Atystar := collect(expand(add(TotalDiff((-1)^j\ Aty \| j \cdot f[0], [j]), j = 0..4)), [f[4], f[3], f[2], f[1], f[0]]);$

$Atzstar := collect(expand(add(TotalDiff((-1)^j\ Atz \| j \cdot f[0], [j]), j = 0..4)), [f[4], f[3], f[2], f[1], f[0]]);$

$Atustar := collect(expand(add(TotalDiff((-1)^j\ Atu \| j \cdot f[0], [j]), j = 0..4)), [f[4], f[3], f[2], f[1], f[0]]);$

$Amystar := collect(expand(add(TotalDiff((-1)^j\ Amy \| j \cdot f[0], [j]), j = 0..4)), [f[4], f[3], f[2], f[1], f[0]]);$

$Amzstar := collect(expand(add(TotalDiff((-1)^j\ Amz \| j \cdot f[0], [j]), j = 0..4)), [f[4], f[3], f[2], f[1], f[0]]);$

$Amustar := collect(expand(add(TotalDiff((-1)^j\ Amu \| j \cdot f[0], [j]), j = 0..4)), [f[4], f[3], f[2], f[1], f[0]]);$

$$Akystar := \left(K_0^2 - T_0^2\right) f_0 + f_2$$

$$Akzstar := 2\, T_0 f_1 + T_1 f_0$$

$$Akustar := M_0\, T_0 f_0$$

$$Atystar := \frac{2\, T_0 f_2}{K_0} + \left(\frac{T_1}{K_0} - \frac{2\, K_1\, T_0}{K_0^2}\right) f_1 + \left(2\, K_0\, T_0 - \frac{M_0^2\, T_0}{K_0}\right) f_0$$

$$Atzstar := -\frac{f_3}{K_0} + \frac{2\, K_1 f_2}{K_0^2} + \left(\frac{3\, M_0^2}{K_0} + \frac{T_0^2}{K_0} - \frac{2\, K_1^2}{K_0^3} + \frac{K_2}{K_0^2} - K_0\right) f_1 + \left(-K_1 + \frac{3\, M_0\, M_1}{K_0} - \frac{2\, K_1\, M_0^2}{K_0^2}\right) f_0$$

$$Atustar := -\frac{3\, M_0 f_2}{K_0} + \left(-\frac{3\, M_1}{K_0} + \frac{4\, K_1\, M_0}{K_0^2}\right) f_1 + \left(-K_0\, M_0 + \frac{M_0^3}{K_0} - \frac{M_2}{K_0} + \frac{2\, K_1\, M_1}{K_0^2}\right.$$

$$- \frac{2 K_1^2 M_0}{K_0^3} + \frac{K_2 M_0}{K_0^2} \Bigg) f_0$$

$$Amystar := \frac{3 M_0 f_2}{K_0} + \left( - \frac{2 K_1 M_0}{K_0^2} + \frac{2 M_1}{K_0} - \frac{2 M_0 T_1}{K_0 T_0} \right) f_1 + \left( \frac{T_0^2 M_0}{K_0} + K_0 M_0 \right) f_0$$

$$Amzstar := - \frac{3 M_0 f_3}{K_0 T_0} + \left( \frac{4 M_0 K_1}{K_0^2 T_0} + \frac{6 T_1 M_0}{K_0 T_0^2} - \frac{3 M_1}{K_0 T_0} \right) f_2 + \Bigg( \frac{3 T_1 M_1}{K_0 T_0^2} + \frac{2 K_1 M_1}{K_0^2 T_0}$$
$$+ \frac{K_2 M_0}{K_0^2 T_0} - \frac{M_2}{K_0 T_0} - \frac{K_0 M_0}{T_0} - \frac{2 K_1^2 M_0}{K_0^3 T_0} - \frac{4 K_1 T_1 M_0}{K_0^2 T_0^2} - \frac{6 T_1^2 M_0}{K_0 T_0^3} + \frac{3 M_0 T_2}{K_0 T_0^2}$$
$$- \frac{T_0 M_0}{K_0} + \frac{M_0^3}{K_0 T_0} \Bigg) f_1 + \left( - \frac{2 M_0 T_1}{K_0} - \frac{M_1 T_0}{K_0} + \frac{2 M_0 T_0 K_1}{K_0^2} \right) f_0$$

$$Amustar := \frac{f_4}{K_0 T_0} + \left( - \frac{3 T_1}{K_0 T_0^2} - \frac{2 K_1}{K_0^2 T_0} \right) f_3 + \Bigg( \frac{2 K_1^2}{K_0^3 T_0} - \frac{K_2}{K_0^2 T_0} + \frac{6 T_1^2}{K_0 T_0^3} - \frac{3 T_2}{K_0 T_0^2} \qquad \mathbf{(5.17)}$$
$$+ \frac{K_0}{T_0} + \frac{T_0}{K_0} - \frac{3 M_0^2}{K_0 T_0} + \frac{4 K_1 T_1}{K_0^2 T_0^2} \Bigg) f_2 + \Bigg( - \frac{K_0 T_1}{T_0^2} - \frac{6 T_1^3}{K_0 T_0^4} - \frac{T_3}{K_0 T_0^2} + \frac{2 T_1}{K_0}$$
$$+ \frac{K_1}{T_0} - \frac{2 K_1 T_0}{K_0^2} - \frac{3 M_0 M_1}{K_0 T_0} + \frac{2 M_0^2 K_1}{K_0^2 T_0} + \frac{3 T_1 M_0^2}{K_0 T_0^2} - \frac{4 K_1 T_1^2}{K_0^2 T_0^3} + \frac{2 K_1 T_2}{K_0^2 T_0^2}$$
$$- \frac{2 K_1^2 T_1}{K_0^3 T_0^2} + \frac{K_2 T_1}{K_0^2 T_0^2} + \frac{6 T_1 T_2}{K_0 T_0^3} \Bigg) f_1 + \Bigg( \frac{T_2}{K_0} - \frac{T_0 K_2}{K_0^2} - \frac{2 K_1 T_1}{K_0^2} - \frac{M_0^2 T_0}{K_0}$$
$$+ \frac{2 K_1^2 T_0}{K_0^3} \Bigg) f_0$$

> $Bystar := -K[0] f[0] : Bzstar := 0 : Bustar := 0 :$

>

# Computing examples of SE(4)-invariant EL eqs

> $DGsetup([s], [K, T, M, seq(ICy \| i, i = 0..4), seq(ICz \| i, i = 0..4), seq(ICu \| i, i = 0..4), f], G, 5) :$

Lagrangian = ds

> $EL0y := eval(Bystar, [f[0] = 1, seq(f[l] = 0, l = 1..4)]) = 0; EL0z := eval(Bzstar, [f[0] = 1, seq(f[l] = 0, l = 1..4)]) = 0; EL0u := eval(Bustar, [f[0] = 1, seq(f[l] = 0, l = 1..4)]) = 0$

$$EL0y := -K_0 = 0$$
$$EL0z := 0 = 0$$
$$EL0u := 0 = 0 \qquad \mathbf{(5.18)}$$

Lagrangian = kappa ds

> $EL1y := simplify(eval(Akystar, [f[0] = 1, seq(f[l] = 0, l = 1..4)]) + eval(Bystar,$

$[seq(f[l] = K[l], l = 0 ..4)])); EL1z := simplify(eval(Akzstar, [f[0] = 1, seq(f[l] = 0, l = 1 ..4)]) + eval(Bzstar, [seq(f[l] = K[l], l = 0 ..4)])); EL1u := simplify(eval(Akustar, [f[0] = 1, seq(f[l] = 0, l = 1 ..4)]) + eval(Bustar, [seq(f[l] = K[l], l = 0 ..4)]))$

$$EL1y := -T_0^2$$

$$EL1z := T_1$$

$$EL1u := M_0 T_0 \quad \textbf{(5.19)}$$

Lagrangian = tau ds

> $EL2y := simplify(eval(Atystar, [f[0] = 1, seq(f[l] = 0, l = 1 ..4)]) + eval(Bystar, [seq(f[l] = T[l], l = 0 ..4)])); EL2z := simplify(eval(Atzstar, [f[0] = 1, seq(f[l] = 0, l = 1 ..4)]) + eval(Bzstar, [seq(f[l] = T[l], l = 0 ..4)])); EL2u := simplify(eval(Atustar, [f[0] = 1, seq(f[l] = 0, l = 1 ..4)]) + eval(Bustar, [seq(f[l] = T[l], l = 0 ..4)]))$

$$EL2y := \frac{T_0 \left(K_0^2 - M_0^2\right)}{K_0}$$

$$EL2z := \frac{-K_1 K_0^2 + 3 M_0 M_1 K_0 - 2 K_1 M_0^2}{K_0^2}$$

$$EL2u := \frac{-K_0^4 M_0 + M_0^3 K_0^2 - M_2 K_0^2 + 2 K_1 M_1 K_0 + K_2 M_0 K_0 - 2 K_1^2 M_0}{K_0^3} \quad \textbf{(5.20)}$$

Lagrangian = mu ds

> $EL3y := simplify(eval(Amystar, [f[0] = 1, seq(f[l] = 0, l = 1 ..4)]) + eval(Bystar, [seq(f[l] = M[l], l = 0 ..4)])); EL3z := simplify(eval(Amzstar, [f[0] = 1, seq(f[l] = 0, l = 1 ..4)]) + eval(Bzstar, [seq(f[l] = M[l], l = 0 ..4)])); EL3u := simplify(eval(Amustar, [f[0] = 1, seq(f[l] = 0, l = 1 ..4)]) + eval(Bustar, [seq(f[l] = M[l], l = 0 ..4)]))$

$$EL3y := \frac{T_0^2 M_0}{K_0}$$

$$EL3z := \frac{-2 M_0 T_1 K_0 - M_1 T_0 K_0 + 2 M_0 T_0 K_1}{K_0^2}$$

$$EL3u := \frac{-M_0^2 T_0 K_0^2 + T_2 K_0^2 - 2 K_1 T_1 K_0 - T_0 K_2 K_0 + 2 K_1^2 T_0}{K_0^3} \quad \textbf{(5.21)}$$

> $solve([EL3y, EL3z, EL3u], [M[0], M[1], T[2]])[1]$

$$\left[M_0 = 0, M_1 = 0, T_2 = \frac{2 K_1 T_1 K_0 + T_0 K_2 K_0 - 2 K_1^2 T_0}{K_0^2}\right] \quad \textbf{(5.22)}$$

Lagrangian = kappa^2 ds

> $EL4y := simplify(eval(Akystar, [seq(f[l] = 2 K[l], l = 0 ..4)]) + eval(Bystar, [seq(f[l] = TotalDiff(K[0]^2, [l]), l = 0 ..4)])); EL4z := simplify(eval(Akzstar, [seq(f[l] = 2 K[l], l = 0 ..4)]) + eval(Bzstar, [seq(f[l] = TotalDiff(K[0]^2, [l]), l = 0 ..4)])); EL4u := simplify(eval(Akustar, [seq(f[l] = 2 K[l], l = 0 ..4)]) + eval(Bustar,$

$[seq(f[l] = TotalDiff(K[0]^2, [l]), l = 0..4)]))$

$$EL4y := K_0^3 - 2\,K_0\,T_0^2 + 2\,K_2$$

$$EL4z := 2\,K_0\,T_1 + 4\,K_1\,T_0$$

$$EL4u := 2\,M_0\,T_0\,K_0 \qquad (5.23)$$

> solve([EL4y, EL4z, EL4u], [K[2], T[1], M[0]])[1] # elastica EL eqn

$$\left[K_2 = K_0\,T_0^2 - \frac{1}{2}\,K_0^3,\ T_1 = -\frac{2\,K_1\,T_0}{K_0},\ M_0 = 0\right] \qquad (5.24)$$

Lagrangian = tau^2 ds

> EL5y := simplify(eval(Atystar, [seq(f[l] = 2 T[l], l = 0..4)]) + eval(Bystar, [seq(f[l] = TotalDiff(T[0]^2, [l]), l = 0..4)])); EL5z := simplify(eval(Atzstar, [seq(f[l] = 2 T[l], l = 0..4)]) + eval(Bzstar, [seq(f[l] = TotalDiff(T[0]^2, [l]), l = 0..4)])); EL5u := simplify(eval(Atustar, [seq(f[l] = 2 T[l], l = 0..4)]) + eval(Bustar, [seq(f[l] = TotalDiff(T[0]^2, [l]), l = 0..4)]))

$$EL5y := \frac{3\,K_0^3\,T_0^2 + \left(-2\,M_0^2\,T_0^2 + 4\,T_0\,T_2 + 2\,T_1^2\right)K_0 - 4\,K_1\,T_0\,T_1}{K_0^2}$$

$$EL5z := \frac{1}{K_0^3}\Big(-2\,K_0^4\,T_1 - 2\,K_0^3\,K_1\,T_0 + \left(\left(6\,M_0^2 + 2\,T_0^2\right)T_1 + 6\,M_0\,T_0\,M_1 - 2\,T_3\right)K_0^2 + \left(2\,K_2\,T_1 - 4\,K_1\left(M_0^2\,T_0 - T_2\right)\right)K_0 - 4\,K_1^2\,T_1\Big)$$

$$EL5u := \frac{1}{K_0^3}\Big(-2\,K_0^4\,M_0\,T_0 + \left(2\,M_0^3\,T_0 - 6\,M_0\,T_2 - 6\,M_1\,T_1 - 2\,M_2\,T_0\right)K_0^2 + \left(\left(8\,K_1\,T_1 + 2\,K_2\,T_0\right)M_0 + 4\,T_0\,K_1\,M_1\right)K_0 - 4\,K_1^2\,M_0\,T_0\Big) \qquad (5.25)$$

> solve([EL5y, EL5z, EL5u], [T[3], K[2], T[2]])[1]

$$\Big[T_3 = -\frac{1}{4\,T_0^2\,M_0\,K_0^2}\big(9\,K_0^4\,M_0\,T_0^2\,T_1 + 10\,K_0^3\,K_1\,M_0\,T_0^3 - 14\,K_0^2\,M_0^3\,T_0^2\,T_1 - 12\,K_0^2\,M_0^2\,M_1\,T_0^3 - 4\,K_0^2\,M_0\,T_0^4\,T_1 + 4\,K_0\,K_1\,M_0^3\,T_0^3 + 6\,K_0^2\,M_0\,T_1^3 - 12\,K_0^2\,M_1\,T_0\,T_1^2 - 4\,K_0^2\,M_2\,T_0^2\,T_1 + 8\,K_0\,K_1\,M_0\,T_0\,T_1^2 + 8\,K_0\,K_1\,M_1\,T_0^2\,T_1 - 8\,K_1^2\,M_0\,T_0^2\,T_1\big),\ K_2 = -\frac{1}{4\,T_0^2\,M_0\,K_0}\big(5\,K_0^4\,M_0\,T_0^2 - 2\,K_0^2\,M_0^3\,T_0^2 + 6\,K_0^2\,M_0\,T_1^2 - 12\,K_0^2\,M_1\,T_0\,T_1 - 4\,K_0^2\,M_2\,T_0^2 + 4\,K_0\,K_1\,M_0\,T_0\,T_1 + 8\,K_0\,K_1\,M_1\,T_0^2 - 8\,K_1^2\,M_0\,T_0^2\big),\ T_2 = -\frac{3\,K_0^3\,T_0^2 - 2\,K_0\,M_0^2\,T_0^2 + 2\,K_0\,T_1^2 - 4\,K_1\,T_0\,T_1}{4\,T_0\,K_0}\Big] \qquad (5.26)$$

Lagrangian = (1 + kappa) ds

> EL6y := simplify(eval(Akystar, [f[0] = 1, seq(f[l] = 0, l = 1..4)]) + eval(Bystar, [f[0]

$= 1 + K[0], seq(f[l] = K[l], l = 1..4)])); EL6z := simplify(eval(Akzstar, [f[0] = 1, seq(f[l] = 0, l = 1..4)]) + eval(Bzstar, [f[0] = 1 + K[0], seq(f[l] = K[l], l = 1..4)])); EL6u := simplify(eval(Akustar, [f[0] = 1, seq(f[l] = 0, l = 1..4)]) + eval(Bustar, [f[0] = 1 + K[0], seq(f[l] = K[l], l = 1..4)]))$

$$EL6y := -T_0^2 - K_0$$

$$EL6z := T_1$$

$$EL6u := M_0 T_0 \quad (5.27)$$

**Global invariant Lagrangian example:**

Lagrangian = K[0]^(-1) K[1]^(-1) ds, Eulerian = -2 K[0]^-2 K[1]^-1 - 2 K[2] K[0]^-1 K[1]^-3 , Hamiltonian = - 2 K[0]^-1 K[1]^-1

> $EL7y := simplify\left(eval\left(Akystar, \left[seq\left(f[l] = TotalDiff\left(-\frac{2}{K[0]^2 K[1]} - \frac{2K[2]}{K[0]K[1]^3}, [l]\right), l = 0..5\right)\right]\right) + eval\left(Bystar, \left[seq\left(f[l] = TotalDiff\left(-\frac{2}{K[0]K[1]}, [l]\right), l = 0..5\right)\right]\right)\right) : EL7z := simplify\left(eval\left(Akzstar, \left[seq\left(f[l] = TotalDiff\left(-\frac{2}{K[0]^2 K[1]} - \frac{2K[2]}{K[0]K[1]^3}, [l]\right), l = 0..5\right)\right]\right) + eval\left(Bzstar, \left[seq\left(f[l] = TotalDiff\left(-\frac{2}{K[0]K[1]}, [l]\right), l = 0..5\right)\right]\right)\right) : EL7u := simplify\left(eval\left(Akustar, \left[seq\left(f[l] = TotalDiff\left(-\frac{2}{K[0]^2 K[1]} - \frac{2K[2]}{K[0]K[1]^3}, [l]\right), l = 0..5\right)\right]\right) + eval\left(Bustar, \left[seq\left(f[l] = TotalDiff\left(-\frac{2}{K[0]K[1]}, [l]\right), l = 0..5\right)\right]\right)\right) :$

> $solve([EL7y, EL7z, EL7u], [K[4], M[0], T[1]])[1]$

$$\left[K_4 = \frac{1}{K_1^2 K_0^3}\left(-K_0^5 K_1^2 K_2 + K_0^3 K_1^2 K_2 T_0^2 + K_0^2 K_1^4 T_0^2 + 9 K_0^3 K_1 K_2 K_3 - 12 K_0^3 K_2^3 + 3 K_0^2 K_1^3 K_3 - 7 K_0^2 K_1^2 K_2^2 - 4 K_0 K_1^4 K_2 - 6 K_1^6\right), M_0 = 0, T_1 = -\frac{2 T_0 \left(K_3 K_0^2 K_1 - 3 K_0^2 K_2^2 - 2 K_2 K_0 K_1^2 - 2 K_1^4\right)}{K_1 K_0 \left(K_2 K_0 + K_1^2\right)}\right] \quad (5.28)$$

We express these conformally invariant EL in terms of the global invariants:

> $DGsetup([s], [K, T, M, P, R, S, Q], H)$ :
*# K,T,M are the local invariants, P,R,S are the global invariants for SE(4)*

> $Nabla := f \to K[0] \cdot K[1] \cdot TotalDiff(f, [1])$# *global invariant derivation (TotalDiff is wrt Ds)*

$$\nabla := f \mapsto K_0 \cdot K_1 \cdot TotalDiff(f, [1]) \quad (5.29)$$

> $nablatods := [P[0] = K[0]^2, R[0] = T[0]^2, S[0] = K[0]^3 T[0]^2 M[0]]$ :
**for** $i$ **from** 1 **to** 15 **do**:
$nablatods := simplify([op(nablatods), P[i] = Nabla(rhs(nablatods[-3])), R[i]$

$= Nabla(rhs(nablatods[-2])), S[i] = Nabla(rhs(nablatods[-1]))], symbolic):$
**end do**:

> $localtoglobal\_sub := simplify(solve(nablatods[1..15], [M[4], T[4], K[4], M[3], T[3], K[3], M[2], T[2], K[2], M[1], T[1], K[1], M[0], T[0], K[0]]), symbolic)[1]:$

> $simplify(eval([EL7y, EL7z, EL7u], localtoglobal\_sub), symbolic):$

global invariant EL for Lagrangian kappa^-1 kappa_s^-1 omega in terms of global invariants:

> $solve(simplify(eval([EL7y, EL7z, EL7u], localtoglobal\_sub), symbolic), [P[4], R[1], S[0]])[1]$

$$\left[P_4 = \frac{1}{4 P_1^2 P_0^2}\left(-2 P_0^3 P_1^3 P_2 + 2 P_0^2 P_1^5 + 2 P_0^2 P_1^3 P_2 R_0 + 32 P_0^2 P_1 P_2 P_3 - 40 P_0^2 P_2^3 - 4 P_0 P_1^3 P_3 + 9 P_0 P_1^2 P_2^2 + P_1^4 P_2\right), R_1 = -\frac{2 R_0 \left(2 P_0 P_1 P_3 - 5 P_0 P_2^2 + P_1^2 P_2\right)}{P_2 P_1 P_0}, S_0 = 0\right] \quad (5.30)$$

# Computing W:

> $DGsetup([x], [y, z, u], E, 12):$

> $\text{omega} := evalDG\left(\frac{1}{Ts(x)} dx\right): \# \textit{ ds, arclength parameter}$

> $vt1 := evalDG\left(\frac{1}{Ts(x)^2} \left( diff(\text{kappa}, y[2]) \cdot (dy[0] - y[1] dx) + diff(\text{kappa}, z[2]) \cdot (dz[0] - z[1] dx) + diff(\text{kappa}, u[2]) \cdot (du[0] - u[1] dx)\right)\right):$
$vt2 := evalDG\left(\frac{\text{kappa}}{Ts(x)^3} \left(diff(\text{tau}, y[3]) \cdot (dy[0] - y[1] dx) + diff(\text{tau}, z[3]) \cdot (dz[0] - z[1] dx) + diff(\text{tau}, u[3]) \cdot (du[0] - u[1] dx)\right)\right):$
$vt3 := evalDG\left(\text{kappa tau} \cdot \frac{1}{Ts(x)^4} \cdot \left(diff(\text{mu}, y[4]) \cdot (dy[0] - y[1] dx) + diff(\text{mu}, z[4]) \cdot (dz[0] - z[1] dx) + diff(\text{mu}, u[4]) \cdot (du[0] - u[1] dx)\right)\right):$

> $simplify(eval([vt1, vt2, vt3], cs), symbolic)$
*# vt1,vt2,vt3 are invariantizations of theta_y0, theta_z0, theta_u0, respectively.*

$$[0\,dx + dy_0 + 0\,dz_0 + 0\,du_0, 0\,dx + 0\,dy_0 + dz_0 + 0\,du_0, 0\,dx + 0\,dy_0 + 0\,dz_0 + du_0] \quad (5.2.1)$$

> $eq := simplify(DGinfo(evalDG(vt1 \,\&w\, \text{omega} - Wky \cdot (dy[0]-y[1] \cdot dx) \,\&w\, dx - Wkz \cdot (dz[0] -z[1] \cdot dx) \,\&w\, dx - Wku \cdot (du[0] - u[1] \cdot dx) \,\&w\, dx), \text{"CoefficientSet"}), symbolic)$ **union** $simplify(DGinfo(evalDG(vt2 \,\&w\, \text{omega} - Wty \cdot (dy[0]-y[1] \cdot dx) \,\&w\, dx - Wtz \cdot (dz[0]-z[1] \cdot dx) \,\&w\, dx - Wtu \cdot (du[0] - u[1] \cdot dx) \,\&w\, dx), \text{"CoefficientSet"}), symbolic)$ **union** $simplify(DGinfo(evalDG(vt3 \,\&w\, \text{omega} - Wmy \cdot (dy[0]-y[1] \cdot dx) \,\&w\, dx - Wmz \cdot (dz[0] -z[1] \cdot dx) \,\&w\, dx - Wmu \cdot (du[0] - u[1] \cdot dx) \,\&w\, dx), \text{"CoefficientSet"}), symbolic):$

> $solW := simplify(solve(eq, \{Wky, Wkz, Wku, Wty, Wtz, Wtu, Wmy, Wmz, Wmu\}), symbolic):$
$W := Transpose(simplify(Matrix(eval(([[Wky, Wkz, Wku], [Wty, Wtz, Wtu], [Wmy, Wmz, Wmu]]), solW)))):$

> *Determinant*(*W*)

$$u_1^2 + y_1^2 + z_1^2 + 1 \quad \textbf{(5.2.2)}$$

**Conclusion:** Det(W) = length^2, so singular extremals are necessarily of null length. These do not exist for Euclidean signature, but can exist for Lorentzian or split signature. (For example: null geodesics for Minkowski metric.) (Note also that 2D: W = 1, 3D: det(W) = ell, 4D: det(W) = ell^2...)

>
